# Supplementary material for: No more gap-shifting: Stochastic many-body-theory based TDHF for accurate theory of polymethine cyanine dyes
Source: arXiv:2406.09544 source file (2024-06-19)
Supplement: Supplementary file 1 [file flav_vw_si_v6.pdf]

# Supporting Information: No more gap-shifting: Stochastic many-body-theory based TDHF for accurate theory of polymethine cyanine dyes

Nadine C. Bradbury,[1*] Barry Y. Li,[1*] Tucker Allen,[1] Justin R. Caram,[1] and Daniel Neuhauser[1]

[1]*Department of Chemistry and Biochemistry, University of California, Los Angeles, Los Angeles, CA, 90095, USA*

## Contents

**1. Geometry Optimization Scheme Using ORCA 5.0** ........ 2
**2. LUMO and HOMO Densities of Flav-1 and ICG-11** ........ 4
**3. Summary Table of Optical Gaps** ........ 4
**4. Summary Table of LUMO/HOMO Gaps** ........ 5
**5. Summary Table of Orbital and Grid Information Used** ........ 5
**6. Validation of Homemade TD-CAM-LDA0 Routine** ........ 6
**7. Illustration of $N_\beta$ Convergence in Flav-7** ........ 8
**8. Optimized Geometries** ........ 8
Flavylium-1 (Flav-1) ........ 9
Flavylium-3 (Flav-3) ........ 11
Flavylium-5 (Flav-5) ........ 13
LFlavylium-7 (LFlav-7) ........ 15
Flavylium-7 (Flav-7) ........ 17
Flavylium-9 (Flav-9) ........ 19
Indocyanine Green-3 (ICG-3) ........ 21
Indocyanine Green-5 (ICG-5) ........ 23
Indocyanine Green-7 (ICG-7) ........ 25
Indocyanine Green-9 (ICG-9) ........ 27
Indocyanine Green-11 (ICG-11) ........ 29
IR-27 ........ 32
IR-26 ........ 34
**References** ........ 35

## 1. Geometry Optimization Scheme Using ORCA 5.0

Plane-wave and real-space DFT methods are highly sensitive to the molecular geometries in finite systems. Therefore, our initial focus is on obtaining good ground-state geometries using localized atomic basis sets. We employ a 3-stage geometry optimization approach. Firstly, we utilize the $r^2$SCAN-3c method in vacuum to swiftly preprocess the initial geometry.[1,2] Subsequently, we use RI-PBE and def2-TZVP basis with a def2/J auxiliary basis to further optimize the structure.[3,4] Lastly, we advance to the hybrid-GGA level, RIJCOSX-PBE0, incorporating 25% Fock exchange, and expanding the basis to def2-TZVPP. We conduct these operations using the ORCA 5.0 program, and relevant input files and optimized structures are provided below and Section 8.[5,6] For this work, we optimize thirteen positively charged dyes: six traditional Flavylium (Flav) dyes with various polymethine lengths ranging from 1 to 9-carbon bridge, two Flav-7 with modified heterocycles (IR-27 and IR-26), and five Indocyanine Green (ICG) dyes with polymethine bridges ranging from 3 to 11 carbons.

To check the obtained geometries, we perform multiple single-point calculations based on these 3-stage optimized structures: these optimized geometries are taken for ground-state calculation through a homemade Near-gap CAM-LDA0 routine using $dx = dy = dz = 0.4$ a.u. (the grid and orbital parameters for each dye are in Table S3). Further, we calculate two extreme LUMO/HOMO energy gaps using local-density approximation (LDA) and restricted Hartree-Fock (RHF), with intermediate estimates for PBE0 and CAM-LDA0 (Table S2). To further validate the geometries, we check the LUMO and HOMO densities among all these methods to ensure they are visually identical (Figure S1).

***Example ORCA 5.0 Geometry Optimization Input File***

```
* xyzfile +1 1 dye_ini.xyz
%pal nprocs  64 end
%maxcore  3000

%Compound

New_Step
! r2SCAN-3c Opt TightSCF NoTrah NoPop KDIIS SOSCF
%base "dye_r2scan3c"
%scf
MaxIter 1200
DIISMaxEq 35
end
%geom
MaxIter 300
```

```
MaxStep 0.2
TolE 7.5e-6
TolRMSG 1.5e-4
TolMaxG 4.5e-4
TolRMSD 3e-3
TolMaxD 6e-3
end
STEP_END

New_Step
! RI PBE def2-TZVP def2/J D4 Opt TightSCF NoPop NoTrah KDIIS SOSCF
%base "dye_pbe"
%scf
MaxIter 1200
DIISMaxEq 35
end
%geom
MaxIter 300
MaxStep 0.2
end
STEP_END

New_Step
! RIJCOSX PBE0 def2-TZVPP def2/J D4 Opt TightSCF NoPop NoTrah KDIIS SOSCF
%base "dye_pbe0"
%scf
MaxIter 1200
DIISMaxEq 35
end
%geom
MaxIter 300
MaxStep 0.2
end
STEP_END

END
```

## 2. LUMO and HOMO Densities of Flav-1 and ICG-11

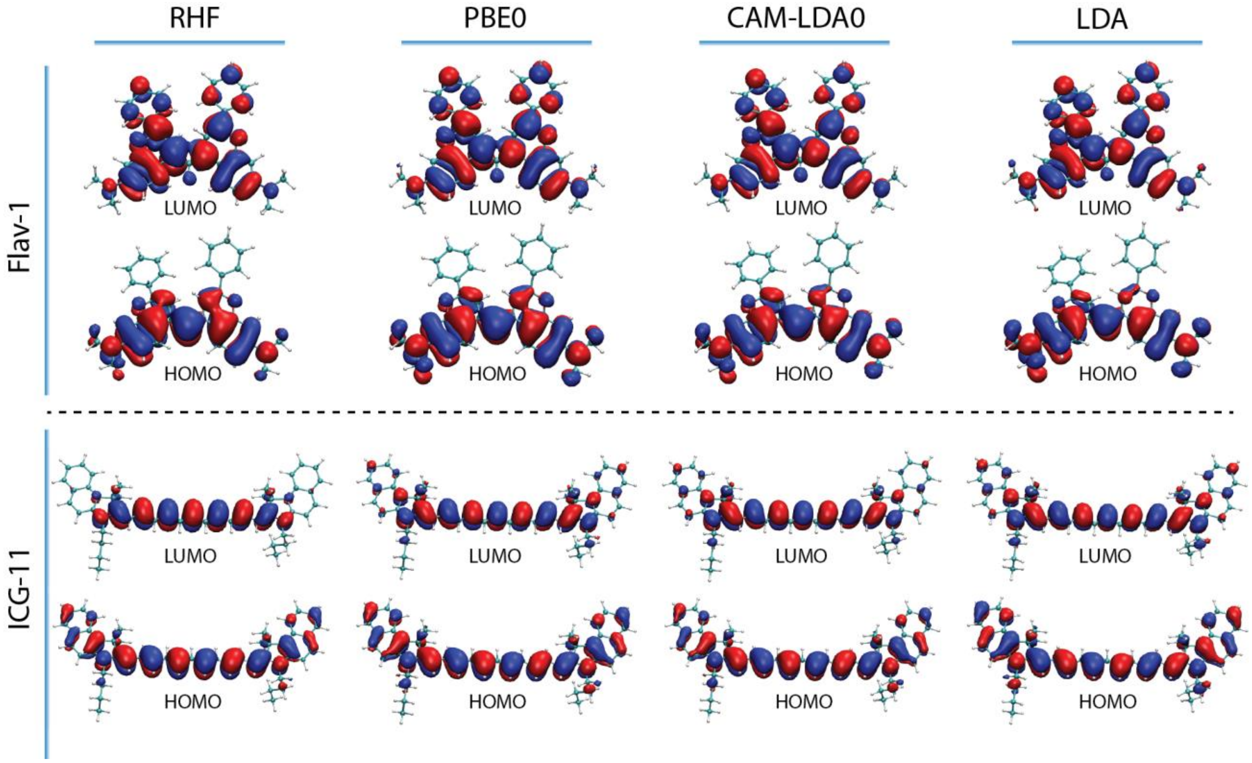


**Figure S1.** LUMO and HOMO densities (isovalue = $\pm 0.016$) for Flav-1, the shortest carbon bridge, and ICG-11, the longest carbon bridge calculated with RHF/def2-TZVPP, PBE0/def2-TZVPP, CAM-LDA0/planewave, and LDA/def2-TZVPP, the orbitals are visually identical. All geometries are taken from PBE0/def2-TZVPP optimized results.

## 3. Summary Table of Optical Gaps

| | TD-LDA | TD-PBE0 | TD-CAM-LDA0 | TD-CAM-B3LYP | TDHF@$v_W$ | Expt. |
|---|---|---|---|---|---|---|
| **Flav-1** | 2.04 | 2.54 | 2.53 | 2.59 | 1.73 | 1.90[7] |
| **Flav-3** | 2.05 | 2.45 | 2.39 | 2.35 | 1.62 | 1.66[7] |
| **Flav-5** | 1.97 | 2.26 | 2.06 | 2.09 | 1.34 | 1.50[7] |
| **LFlav-7** | 1.91 | 2.12 | 2.01 | 1.91 | 1.35 | 1.26[7] |
| **Flav-7** | 1.90 | 2.06 | 1.94 | 1.82 | 1.29 | 1.21[7] |
| **Flav-9** | 1.85 | 2.00 | 1.84 | 1.75 | 1.21 | 1.12[7] |
| **ICG-3** | 2.25 | 2.66 | 2.80 | 2.71 | 2.03 | 2.10[8,9] |
| **ICG-5** | 2.14 | 2.49 | 2.49 | 2.43 | 1.78 | 1.83[10] |
| **ICG-7** | 2.05 | 2.33 | 2.16 | 2.20 | 1.44 | 1.59[10] |
| **ICG-9** | 1.98 | 2.20 | 1.97 | 2.01 | 1.26 | 1.36[11] |
| **ICG-11** | 1.91 | 2.07 | 1.82 | 1.85 | 1.29 | 1.21[11] |
| **IR-27** | 2.16 | 2.15 | 1.95 | 1.85 | 1.29 | 1.26[12] |
| **IR-26** | 2.06 | 2.07 | 1.80 | 1.72 | 1.20 | 1.15[12] |
| **MAE** | 0.55 eV | 0.79 eV | 0.66 eV | 0.63 eV | 0.09 eV | 0.00 eV |
| **Fit Slope** | 0.25 | 0.66 | 0.97 | 1.03 | 0.78 | 1.00 |

**Table S1.** Optical gaps (units: eV) and statistical information calculated from various level of theories.

## 4. Summary Table of LUMO/HOMO Gaps

| | RHF | CAM-LDA0 | PBE0 | LDA |
|---|---|---|---|---|
| **Flav-1** | 7.407 | 4.439 | 2.776 | 1.473 |
| **Flav-3** | 6.874 | 4.074 | 2.498 | 1.332 |
| **Flav-5** | 6.352 | 3.696 | 2.198 | 1.147 |
| **LFlav-7** | 6.019 | 3.500 | 1.998 | 1.025 |
| **Flav-7** | 5.839 | 3.445 | 1.927 | 0.976 |
| **Flav-9** | 5.725 | 3.166 | 1.820 | 0.917 |
| **ICG-3** | 7.676 | 4.714 | 2.906 | 1.379 |
| **ICG-5** | 7.128 | 4.215 | 2.563 | 1.358 |
| **ICG-7** | 6.669 | 3.773 | 2.289 | 1.193 |
| **ICG-9** | 6.293 | 3.499 | 2.070 | 1.059 |
| **ICG-11** | 5.981 | 3.225 | 1.890 | 0.950 |
| **IR-27** | 5.842 | 3.164 | 1.949 | 0.995 |
| **IR-26** | 5.539 | 3.166 | 1.803 | 0.904 |

**Table S2.** LUMO/HOMO gaps (units: eV) calculated from various level of theories, the def2-TZVPP atomic-centered basis set is used for RHF, PBE0, and LDA calculations, and the planewave basis is used for CAM-LDA0.

## 5. Summary Table of Orbital and Grid Information Used

| | $N_{\text{orb}}^{\text{occ}}$ | $N_x$ | $N_{\text{grid}} = N_x \times N_y \times N_z$ |
|---|---|---|---|
| **Flav-1** | 96 | 100 | 800000 |
| **Flav-3** | 101 | 110 | 880000 |
| **Flav-5** | 106 | 140 | 1120000 |
| **LFlav-7** | 111 | 140 | 1120000 |
| **Flav-7** | 122 | 140 | 1120000 |
| **Flav-9** | 116 | 160 | 1280000 |
| **ICG-3** | 105 | 110 | 880000 |
| **ICG-5** | 110 | 120 | 960000 |
| **ICG-7** | 115 | 130 | 1040000 |
| **ICG-9** | 120 | 130 | 1040000 |
| **ICG-11** | 125 | 150 | 1200000 |
| **IR-27** | 104 | 140 | 1120000 |
| **IR-26** | 104 | 140 | 1120000 |

**Table S3.** Number of occupied molecular orbitals, the number of $x$-grid, and the total number of grid points used for each dye molecule, $N_y = 100$ and $N_z = 80$ are used and held constant throughout the computations.

## 6. Validation of Homemade TD-CAM-LDA0 Routine

Spectroscopic validations of TD-CAM-LDA0 implementation of the homemade Near-gap TDDFT code. ORCA 5.0.4 program is used for TDDFT calculation at CAM-B3LYP/def2-TZVPP level of theory with fixed PBE0/def2-TZVPP optimized geometries, CAM-B3LYP is considered as the closest commercially available functional compared to the TD Near-gap treatment.[1–6] The ORCA-calculated oscillator strengths of the lowest-energy excitation were converted to absorption cross-sections (with broadened Gaussian FWHM = 0.016 eV for each) for convenient comparison.

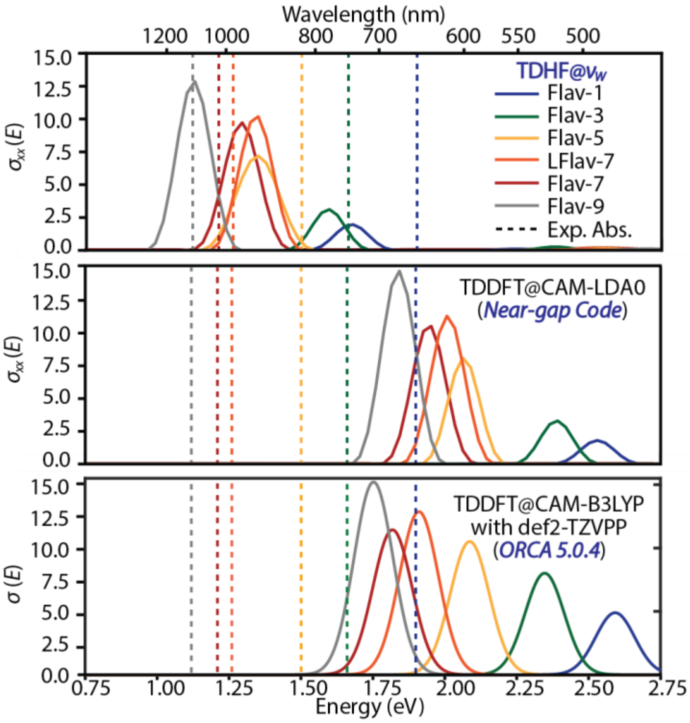


**Figure S2.** Spectra for Flav series calculated using TDHF@$v_W$ (top), TDDFT@CAM-LDA0 homemade code (middle), and TDDFT@CAM-B3LYP with def2-TZVPP basis set in ORCA program (bottom).

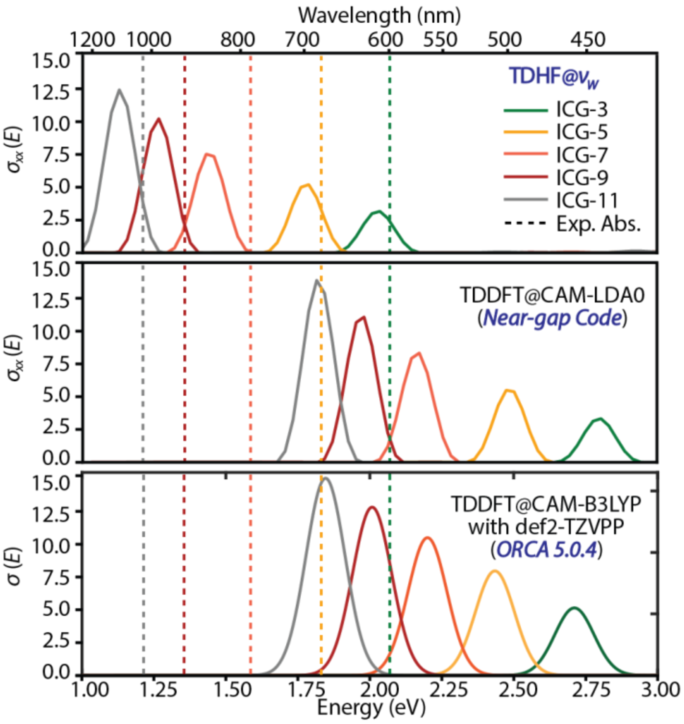


**Figure S3.** Spectra for ICG series calculated using TDHF@$v_W$ (top), TDDFT@CAM-LDA0 homemade code (middle), and TDDFT@CAM-B3LYP with def2-TZVPP basis set in ORCA program (bottom).

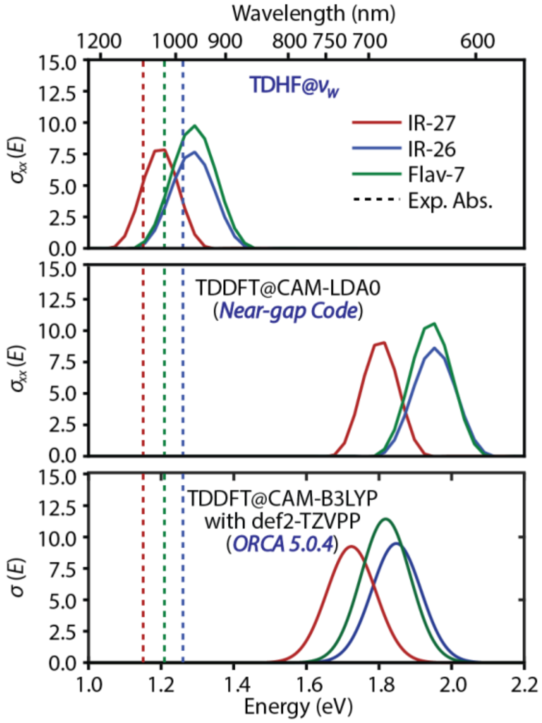


**Figure S4.** Spectra for IR-27, IR-26, and Flav-7 calculated using TDHF@$v_W$ (top), TDDFT@CAM-LDA0 homemade code (middle), and TDDFT@CAM-B3LYP with def2-TZVPP basis set in ORCA program (bottom).

## 7. Illustration of $N_\beta$ Convergence in Flav-7

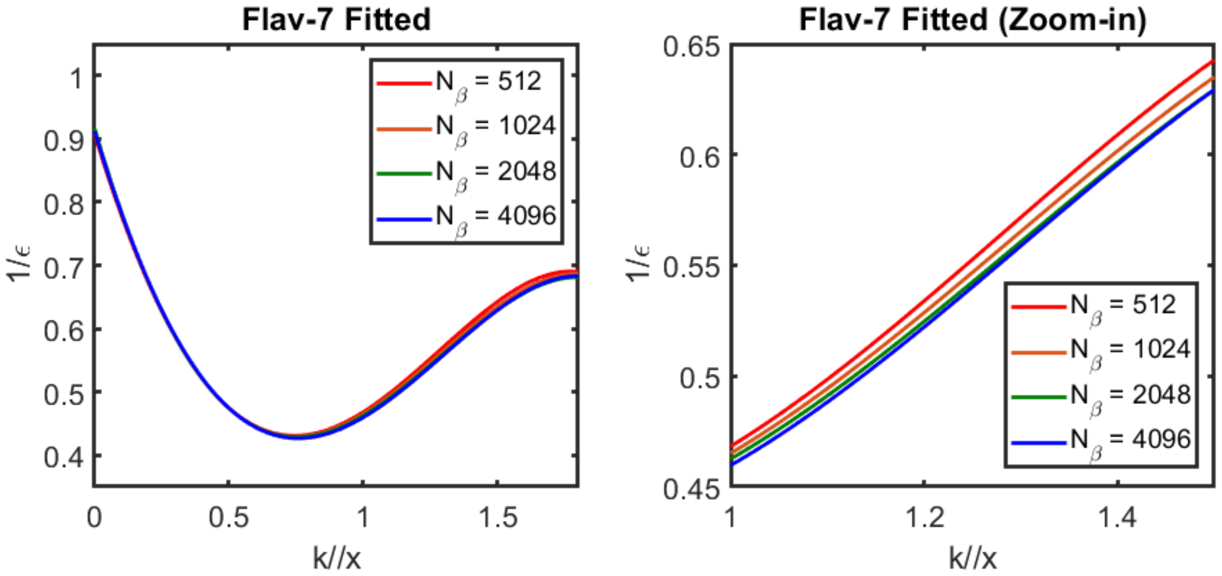


**Figure S5.** Fitted $\epsilon^{-1} = 1 + v_W^{pol}(k_x)/v(k_x)$ for Flav-7 with different numbers of samplers, i.e., $N_\beta$ ranged from $2^9$ to $2^{12}$. The fittings show nice convergence, and the number of samplers does not significantly affect the overall fitting results.

## 8. Optimized Geometries

All final geometries are optimized at PBE0/def2-TZVPP level in vacuum, with +1*e* charge for each dye. The coordinates are in *.xyz* format and in unit of Å.

Flavylium-1 (Flav-1)

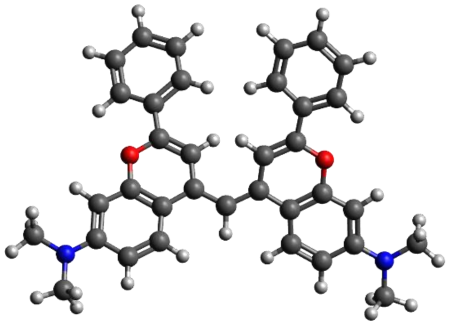

| | | | |
|---|---|---|---|
| 70 | | | |
| C | 0.2381871088 | 4.7498556593 | 5.2744071211 |
| O | 1.1950226635 | 5.3890923759 | 4.5890839782 |
| C | 1.5223022342 | 4.9936311666 | 3.3332375258 |
| C | 0.8310514342 | 3.9524565036 | 2.6948604942 |
| C | -0.2407042138 | 3.2947200728 | 3.3832202849 |
| C | -0.4770924813 | 3.7431195161 | 4.7103655519 |
| C | 0.0951449160 | 5.2254027460 | 6.6466962920 |
| C | 2.5546513004 | 5.6906729779 | 2.7453288696 |
| C | 1.2411675399 | 3.6639732567 | 1.3809885890 |
| H | -1.1692268437 | 3.2066962471 | 5.3371007408 |
| C | 2.9655651186 | 5.3687256998 | 1.4449269314 |
| C | 2.2635732152 | 4.3325069826 | 0.7723789632 |
| H | 3.0235335862 | 6.4784465760 | 3.3148847264 |
| N | 3.9854894962 | 6.0216326889 | 0.8467288855 |
| H | 0.7236945185 | 2.8979086122 | 0.8196658873 |
| H | 2.5292776430 | 4.0705861547 | -0.2408480388 |
| C | -0.9307133407 | 2.2199395696 | 2.8150755738 |
| C | -2.1691060569 | 1.6997150392 | 3.2033596994 |
| C | -3.1169012421 | 2.4473692948 | 3.9520863760 |
| C | -4.3422300127 | 1.9543601697 | 4.2678340725 |
| O | -4.7113670985 | 0.7225607320 | 3.8949084376 |
| C | -3.8815871830 | -0.0501139812 | 3.1500052965 |
| C | -2.6045089736 | 0.4004679514 | 2.7828962703 |
| H | -2.9110336691 | 3.4757266704 | 4.1962943746 |
| C | -5.3841480069 | 2.6705517145 | 4.9966094097 |
| C | -1.8246788473 | -0.5087351292 | 2.0462104467 |
| C | -4.3763534880 | -1.2890196310 | 2.8064857590 |
| C | -2.2863862180 | -1.7420071455 | 1.6883428968 |
| C | -3.5902669747 | -2.1716952191 | 2.0536702909 |
| H | -0.8164977580 | -0.2368190058 | 1.7648539388 |
| H | -1.6389447909 | -2.4002965787 | 1.1286515649 |
| H | -5.3703085327 | -1.5486129654 | 3.1374069758 |
| N | -4.0470884185 | -3.3909538692 | 1.6945919729 |
| C | 4.6688459031 | 7.0832808090 | 1.5465627475 |
| C | 4.3892197583 | 5.6797553355 | -0.4978860035 |
| C | -5.3688280587 | -3.8110125224 | 2.0941520054 |
| C | -3.2164096465 | -4.2888418932 | 0.9250561151 |
| H | 5.1180860140 | 6.7230967317 | 2.4769859321 |

| | | | |
|---|---|---|---|
| H | 3.9915510244 | 7.9087241063 | 1.7871214594 |
| H | 5.4649517311 | 7.4724218275 | 0.9181909144 |
| H | 4.6852430871 | 4.6298449059 | -0.5732577174 |
| H | 5.2458705403 | 6.2873996508 | -0.7758797872 |
| H | 3.5919860187 | 5.8691093554 | -1.2229137317 |
| H | -2.3068496438 | -4.5650777338 | 1.4666914320 |
| H | -2.9293298870 | -3.8489842702 | -0.0341209663 |
| H | -3.7733561417 | -5.1990729139 | 0.7212370778 |
| H | -5.4700974150 | -3.8362932172 | 3.1836031202 |
| H | -5.5564600069 | -4.8118403761 | 1.7157683550 |
| H | -6.1391963292 | -3.1464692461 | 1.6910977856 |
| C | 1.0662943409 | 6.0584306130 | 7.2054155345 |
| C | 0.9451766490 | 6.4952752544 | 8.5125739309 |
| C | -0.1446885440 | 6.1120294907 | 9.2792475074 |
| C | -1.1191224113 | 5.2889015908 | 8.7301877471 |
| C | -1.0023279305 | 4.8500125215 | 7.4256666589 |
| H | 1.9213913782 | 6.3551542755 | 6.6145568346 |
| H | 1.7081610222 | 7.1360443483 | 8.9359511505 |
| H | -0.2370639126 | 6.4545225794 | 10.3022331120 |
| H | -1.9752074546 | 4.9905789240 | 9.3220367989 |
| H | -1.7788049450 | 4.2187471197 | 7.0132582274 |
| C | -5.0965523766 | 3.8545777578 | 5.6801392137 |
| C | -6.0905905937 | 4.5287056875 | 6.3626129658 |
| C | -7.3875944811 | 4.0327669922 | 6.3760965413 |
| C | -7.6826101421 | 2.8564396636 | 5.7038583220 |
| C | -6.6899118407 | 2.1769545957 | 5.0206383516 |
| H | -4.0895095694 | 4.2508592754 | 5.6926814262 |
| H | -5.8533960080 | 5.4435365951 | 6.8907279994 |
| H | -8.1653196461 | 4.5625390671 | 6.9116056396 |
| H | -8.6922961343 | 2.4659310233 | 5.7096463063 |
| H | -6.9260653938 | 1.2625279575 | 4.4949364326 |
| H | -0.4522794804 | 1.7354461999 | 1.9763320705 |

Flavylium-3 (Flav-3)

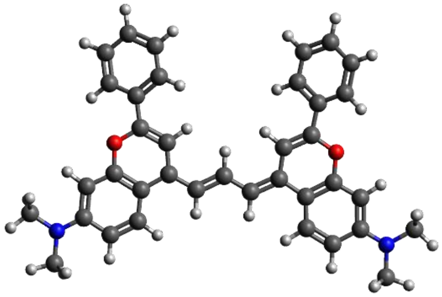

74

| | | | |
|---|---|---|---|
| C | 0.8082553970 | 6.0552644261 | 4.9657638315 |
| O | 1.9397280836 | 6.5249867213 | 4.4212776308 |
| C | 2.5070718006 | 5.8902738986 | 3.3659076147 |
| C | 1.9299086557 | 4.7352118918 | 2.8151986561 |
| C | 0.7235911875 | 4.2114216272 | 3.3848732490 |
| C | 0.2052851019 | 4.9384171115 | 4.4905311910 |
| C | 0.3468758630 | 6.8542695833 | 6.0965880611 |
| C | 3.6619770935 | 6.4659556954 | 2.8843481727 |
| C | 2.6128492368 | 4.1795182751 | 1.7181792673 |
| H | -0.6785555679 | 4.5989147806 | 5.0056015766 |
| C | 0.1052580078 | 3.0601300018 | 2.8850236380 |
| C | 4.3216101175 | 5.8987548833 | 1.7861031020 |
| C | 3.7576724991 | 4.7269164253 | 1.2162579245 |
| H | 4.0250249749 | 7.3571900579 | 3.3729138863 |
| N | 5.4496693878 | 6.4458454975 | 1.2827820808 |
| H | 2.2257608015 | 3.2880343633 | 1.2450552149 |
| H | 4.2349483091 | 4.2540625126 | 0.3709202407 |
| C | -1.0712539111 | 2.5092391015 | 3.3613019407 |
| C | -1.6655844872 | 1.3785996824 | 2.8289661519 |
| C | -2.8699572587 | 0.8142322982 | 3.2630570703 |
| H | 0.5712709393 | 2.5555595748 | 2.0480023638 |
| H | -1.5610287920 | 2.9976905229 | 4.1959176561 |
| H | -1.1543270919 | 0.9084448040 | 1.9983376856 |
| C | -3.6307872485 | 1.3656089195 | 4.3291496481 |
| C | -4.8103625717 | 0.8294266028 | 4.7258560962 |
| O | -5.3276625308 | -0.2495137362 | 4.1214062615 |
| C | -4.6640109111 | -0.8456882601 | 3.0999611130 |
| C | -3.4313661304 | -0.3508013552 | 2.6450277912 |
| H | -3.3024970789 | 2.2594515193 | 4.8340979995 |
| C | -5.6579793772 | 1.3456093480 | 5.7957947632 |
| C | -2.8449771645 | -1.0647174947 | 1.5842139329 |
| C | -5.2833361812 | -1.9524847904 | 2.5626584899 |
| C | -3.4329883489 | -2.1644890841 | 1.0301748721 |
| C | -4.6817047227 | -2.6463530902 | 1.5044516452 |
| H | -1.8931572764 | -0.7422262454 | 1.1859709972 |
| H | -2.9315603518 | -2.6715951783 | 0.2193844187 |
| H | -6.2281266128 | -2.2584459155 | 2.9853313740 |

| | | | |
|---|---|---|---|
| N | -5.2638300118 | -3.7341414638 | 0.9539429115 |
| C | 6.0072620432 | 7.6313368603 | 1.8880512534 |
| C | 6.1204676449 | 5.8389600581 | 0.1560955828 |
| C | -6.5280694107 | -4.2094172561 | 1.4625508946 |
| C | -4.6164129761 | -4.4473485082 | -0.1231437555 |
| H | 6.2897274951 | 7.4556784012 | 2.9308929548 |
| H | 5.3005894432 | 8.4661744003 | 1.8579074374 |
| H | 6.8991426577 | 7.9260029677 | 1.3423198867 |
| H | 6.4596113266 | 4.8241851178 | 0.3846038122 |
| H | 6.9933255930 | 6.4333764790 | -0.0993277058 |
| H | 5.4732309883 | 5.7988165084 | -0.7245799004 |
| H | -3.6456194075 | -4.8483416583 | 0.1828504798 |
| H | -4.4683001177 | -3.8085368164 | -0.9983760460 |
| H | -5.2434284000 | -5.2824629438 | -0.4229010094 |
| H | -6.4540223443 | -4.5020096237 | 2.5147371833 |
| H | -6.8394498040 | -5.0796846227 | 0.8917619011 |
| H | -7.3079293918 | -3.4474306451 | 1.3706300902 |
| C | 1.2460034077 | 7.6570927292 | 6.7997006325 |
| C | 0.8157500486 | 8.4043006341 | 7.8813728251 |
| C | -0.5154873260 | 8.3688594295 | 8.2686908326 |
| C | -1.4185034714 | 7.5822306962 | 7.5667684110 |
| C | -0.9924351866 | 6.8294115230 | 6.4887876238 |
| H | 2.2850805689 | 7.6831607898 | 6.5013047854 |
| H | 1.5232006617 | 9.0174097662 | 8.4251835569 |
| H | -0.8516004560 | 8.9592541936 | 9.1117878121 |
| H | -2.4623315122 | 7.5673270539 | 7.8538340813 |
| H | -1.7115596341 | 6.2468527622 | 5.9270278953 |
| C | -5.1157235874 | 2.1160195682 | 6.8254769727 |
| C | -5.9282775619 | 2.6157403119 | 7.8256960618 |
| C | -7.2914229590 | 2.3537136810 | 7.8124986251 |
| C | -7.8366007481 | 1.5819331782 | 6.7972352227 |
| C | -7.0268532589 | 1.0749690800 | 5.7969284243 |
| H | -4.0488546163 | 2.2964062622 | 6.8633865808 |
| H | -5.4959274273 | 3.2008042271 | 8.6275515843 |
| H | -7.9261757789 | 2.7446876230 | 8.5977569688 |
| H | -8.8989273789 | 1.3735617612 | 6.7845311372 |
| H | -7.4541413801 | 0.4769440130 | 5.0036524314 |

Flavylium-5 (Flav-5)

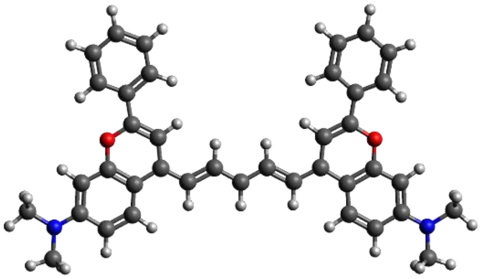

| | | | |
|---|---|---|---|
| 78 | | | |
| C | 0.4292110120 | -0.6612983650 | 0.6575768870 |
| C | 1.7547219630 | -1.0098171370 | 0.8607574940 |
| C | -2.8508391540 | -2.0302856540 | -0.4312132220 |
| C | 2.7642660330 | -0.1498110790 | 1.3082503790 |
| C | 2.5198034860 | 1.2201384350 | 1.6045302530 |
| C | 4.1137695860 | -0.5954177230 | 1.4962478710 |
| C | 3.5014987650 | 2.0482614090 | 2.0352884050 |
| C | 5.0818403080 | 0.3184112100 | 1.9437831730 |
| C | 4.5733739580 | -1.9066727640 | 1.2676561210 |
| C | 6.4031504090 | -0.0123244690 | 2.1504809940 |
| C | 5.8762169150 | -2.2669310530 | 1.4613369150 |
| C | 6.8414247030 | -1.3236505170 | 1.9091366230 |
| H | 3.8799903990 | -2.6635161830 | 0.9268996020 |
| H | 6.1703381000 | -3.2885129650 | 1.2693471650 |
| O | 4.7599679790 | 1.6100153540 | 2.2018284910 |
| N | 8.1284724150 | -1.6807622560 | 2.0932368280 |
| C | 9.0881203660 | -0.7072459500 | 2.5578400730 |
| C | 8.5596276160 | -3.0375280170 | 1.8417877230 |
| H | 8.0457676340 | -3.7523616230 | 2.4913597980 |
| H | 9.6262507520 | -3.1094563300 | 2.0374498050 |
| H | 8.3850699780 | -3.3298279520 | 0.8023183290 |
| H | 9.1841590450 | 0.1278680090 | 1.8567311330 |
| H | 10.0599266690 | -1.1835435510 | 2.6546413390 |
| H | 8.8069421240 | -0.3016964680 | 3.5347922050 |
| H | 5.3942834410 | 3.7048436480 | 2.9907633500 |
| C | 4.4388232020 | 4.1921966130 | 2.8537233140 |
| C | 3.3495437220 | 3.4654660950 | 2.3657428950 |
| C | 2.1241872860 | 4.1176476720 | 2.2004532580 |
| H | 1.2627590130 | 3.5832432810 | 1.8223356180 |
| C | 1.9958907530 | 5.4582921090 | 2.5131941310 |
| H | 1.0398923980 | 5.9491896620 | 2.3769554340 |
| C | 3.0847466790 | 6.1735251100 | 2.9966952450 |
| H | 2.9809714230 | 7.2241663120 | 3.2398472760 |
| C | 4.3041726360 | 5.5347572870 | 3.1661040980 |
| H | 5.1584391450 | 6.0835880360 | 3.5437828690 |
| C | -4.1929241730 | -1.6972625980 | -0.6465145170 |
| C | -4.6988623450 | -0.3865693620 | -0.4210999500 |

| | | | |
|---|---|---|---|
| C | -5.1470658560 | -2.6590939830 | -1.1150988450 |
| C | -5.9995126920 | -0.0736940470 | -0.6344108260 |
| C | -7.4638952520 | -3.1125785590 | -1.7737401110 |
| C | -4.8635857450 | -4.0097368150 | -1.3953911090 |
| C | -7.1600684410 | -4.4560502090 | -2.0432380370 |
| C | -5.8178458720 | -4.8793507970 | -1.8399786940 |
| H | -3.8584856940 | -4.3838614820 | -1.2555418480 |
| H | -5.5392316940 | -5.9043279080 | -2.0372194270 |
| O | -6.8751347900 | -0.9876524220 | -1.0839853450 |
| H | -4.0402469060 | 0.3964697470 | -0.0808618720 |
| H | -4.9609259880 | 2.0562979460 | 0.6956150420 |
| C | -5.9397923240 | 2.2434633690 | 0.2737366790 |
| C | -6.6106507600 | 1.2392636660 | -0.4296767650 |
| C | -7.8847297430 | 1.5058292600 | -0.9370587990 |
| H | -8.4176305370 | 0.7403713690 | -1.4843730840 |
| C | -8.4679028110 | 2.7481345610 | -0.7511381280 |
| H | -9.4548028960 | 2.9411454740 | -1.1541564980 |
| C | -7.7933773250 | 3.7400930970 | -0.0541710120 |
| H | -8.2520415740 | 4.7104089630 | 0.0939555630 |
| C | -6.5277821960 | 3.4817129430 | 0.4576715750 |
| H | -5.9981338760 | 4.2480928070 | 1.0104692790 |
| N | -8.1027672570 | -5.3162013620 | -2.4778806800 |
| C | -9.4568642690 | -4.8585485050 | -2.6839828240 |
| C | -7.7732446450 | -6.6990484850 | -2.7399814340 |
| H | -9.4977011250 | -4.0511679220 | -3.4217125020 |
| H | -9.9038762920 | -4.4941170110 | -1.7535748820 |
| H | -10.0599266690 | -5.6845359860 | -3.0510438110 |
| H | -7.3766252230 | -7.1937779720 | -1.8489332660 |
| H | -7.0369778350 | -6.7945303760 | -3.5437828690 |
| H | -8.6752055540 | -7.2241663120 | -3.0431946300 |
| H | 2.0206394140 | -2.0390567100 | 0.6516308660 |
| C | -0.5422543950 | -1.5462381520 | 0.2104851940 |
| H | 0.1039952040 | 0.3571518580 | 0.8514716850 |
| C | -1.8637494360 | -1.1671590370 | 0.0159330890 |
| H | -0.2576225470 | -2.5751257440 | 0.0042570010 |
| H | -2.1101513370 | -0.1312446560 | 0.2328754930 |
| H | -2.5425221330 | -3.0497163660 | -0.6296104810 |
| C | -6.4779557400 | -2.2619268710 | -1.3245522990 |
| H | -8.4604518720 | -2.7168899200 | -1.9034316770 |
| H | 1.5282251150 | 1.6264872190 | 1.4890131260 |
| H | 7.0747431610 | 0.7599060980 | 2.4960185590 |

LFlavylium-7 (LFlav-7)

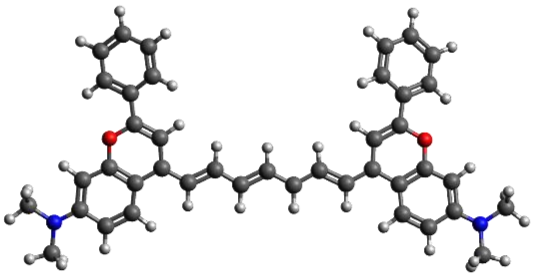

82

| | | | |
|---|---|---|---|
| C | -0.0819853110 | -1.4025090650 | -0.2272938130 |
| C | -1.2380195770 | -2.1666106050 | -0.1950544020 |
| C | 1.1577328220 | -1.8467195610 | -0.6605343260 |
| C | 2.2734183750 | -1.0252353940 | -0.7075141320 |
| C | 3.5286857850 | -1.4304880010 | -1.1280748690 |
| C | -2.4559562160 | -1.6698243200 | 0.2432339380 |
| C | -3.6378780970 | -2.3907733670 | 0.2438689310 |
| H | 2.1278161900 | 0.0022146250 | -0.3857899400 |
| C | 4.6597751160 | -0.6145346560 | -1.2200273880 |
| C | 4.6162680260 | 0.7801168440 | -0.9512564640 |
| C | 5.9400503470 | -1.1256049430 | -1.6170756350 |
| C | 5.7099729800 | 1.5722271680 | -1.0637468780 |
| C | 7.0284523730 | -0.2460324980 | -1.7227287450 |
| O | 6.8972616770 | 1.0752627310 | -1.4449765820 |
| H | 3.6841767660 | 1.2537274380 | -0.6897934530 |
| C | 6.2147341280 | -2.4712280300 | -1.9182907510 |
| C | 8.2916730610 | -0.6447381540 | -2.1015777820 |
| C | 7.4557383980 | -2.8976595200 | -2.2960178620 |
| C | 8.5412132240 | -1.9896748080 | -2.4031303670 |
| H | 5.4232175230 | -3.2043320530 | -1.8475233100 |
| H | 7.6040701750 | -3.9449679160 | -2.5129325970 |
| H | 7.5812299690 | 5.7533382960 | -1.5989384110 |
| C | 6.7853175230 | 5.1590763620 | -1.1680699380 |
| C | 5.7884932720 | 5.7689751740 | -0.4214753260 |
| H | 5.8060259710 | 6.8400589380 | -0.2636587570 |
| C | 4.7723012130 | 5.0010136250 | 0.1306574200 |
| H | 4.0006750970 | 5.4698946470 | 0.7280678330 |
| C | 4.7486733970 | 3.6339112830 | -0.0691360920 |
| H | 3.9677091850 | 3.0430723170 | 0.3918482510 |
| C | 5.7419512640 | 3.0125700550 | -0.8285700280 |
| C | 6.7672288960 | 3.7902172480 | -1.3689709970 |
| H | 7.5427638350 | 3.3187895910 | -1.9566573320 |
| C | -4.8817736980 | -1.9225522980 | 0.6760509510 |
| C | -5.0554640530 | -0.6342383890 | 1.2501225940 |
| C | -6.0743564270 | -2.7117721280 | 0.5614956420 |
| C | -7.2963217810 | -2.1795027590 | 1.0006183230 |
| C | -6.2619949410 | -0.1930093930 | 1.6813113560 |

| | | | |
|---|---|---|---|
| O | -7.3671998120 | -0.9455514620 | 1.5596058460 |
| H | -4.2165474250 | 0.0352256780 | 1.3494041750 |
| C | -8.4952172260 | -2.8521407380 | 0.9044352670 |
| C | -6.1383112570 | -4.0026883420 | 0.0079660590 |
| C | -8.5358466320 | -4.1360679950 | 0.3457108680 |
| C | -7.3099682860 | -4.6955109870 | -0.0999014730 |
| H | -7.2939531470 | -5.6829212680 | -0.5365410860 |
| H | -5.2341391350 | -4.4721901940 | -0.3536381290 |
| H | -7.2188893780 | 4.5648290820 | 3.8814409050 |
| C | -7.0240031950 | 3.5973646190 | 3.4359207730 |
| C | -8.0579623930 | 2.8767271910 | 2.8572609600 |
| H | -9.0617722810 | 3.2822460090 | 2.8450719030 |
| C | -7.8125480350 | 1.6375400190 | 2.2929513570 |
| C | -6.5218089930 | 1.1066363190 | 2.2931546910 |
| C | -5.4885975570 | 1.8355215250 | 2.8850228510 |
| H | -4.4893015670 | 1.4222979610 | 2.9317727950 |
| C | -5.7395157950 | 3.0711962970 | 3.4505814210 |
| H | -4.9322260780 | 3.6223701700 | 3.9160802060 |
| N | -9.6974354110 | -4.8189500380 | 0.2303441120 |
| C | -10.9329066620 | -4.2152566440 | 0.6672850950 |
| C | -9.7189618540 | -6.1337804520 | -0.3673575810 |
| N | 9.7698341490 | -2.4112062920 | -2.7793369190 |
| C | 10.0085546370 | -3.8040942170 | -3.0767695200 |
| C | 10.8549827970 | -1.4656321680 | -2.8773057850 |
| H | -9.3753442880 | -6.1132839020 | -1.4060457530 |
| H | -10.7382231730 | -6.5100875400 | -0.3595411100 |
| H | -9.0964906740 | -6.8400589380 | 0.1892362380 |
| H | -10.9113465420 | -3.9853848500 | 1.7370119130 |
| H | -11.7522923490 | -4.9059221640 | 0.4883936590 |
| H | -11.1434442330 | -3.2900489770 | 0.1211870220 |
| H | 9.8032770930 | -4.4432270620 | -2.2129869470 |
| H | 11.0526493340 | -3.9342545860 | -3.3479207620 |
| H | 9.3978386740 | -4.1498244500 | -3.9160802060 |
| H | 10.6338258660 | -0.6758877910 | -3.6018957100 |
| H | 11.7522923490 | -1.9824192080 | -3.2061580610 |
| H | 11.0684535170 | -0.9960283480 | -1.9117775910 |
| H | -2.4611597780 | -0.6401342190 | 0.5899942730 |
| H | -3.5835329500 | -3.4016207660 | -0.1404658470 |
| H | 3.6293985870 | -2.4712869030 | -1.4094211510 |
| H | 9.0658155180 | 0.1058802030 | -2.1491626650 |
| H | -8.6196892840 | 1.0791527670 | 1.8391864030 |
| H | -9.3826947770 | -2.3589000990 | 1.2705630660 |
| H | -0.1550480620 | -0.3686879190 | 0.1063738000 |
| H | -1.1895605860 | -3.1962930960 | -0.5387025740 |
| H | 1.2555278740 | -2.8789191130 | -0.9855898270 |

Flavylium-7 (Flav-7)

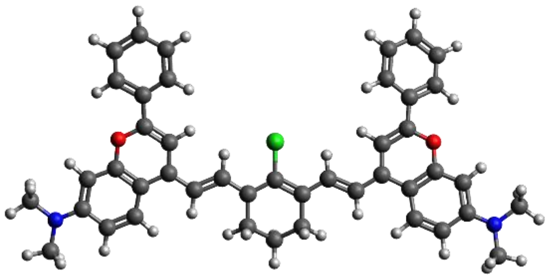

89

| | | | |
|---|---|---|---|
| C | -0.1098273590 | -1.6424551970 | -0.6812886270 |
| C | -1.2739308630 | -2.4220294890 | -0.6523302900 |
| C | 1.1594161210 | -2.1096167760 | -1.0520350070 |
| C | -1.1748461250 | -3.8516756100 | -1.1140217810 |
| C | -0.0147817090 | -4.0734872280 | -2.0615987100 |
| H | -2.1084401300 | -4.1396918930 | -1.6002701650 |
| H | -1.0683144730 | -4.5042907810 | -0.2392263060 |
| C | 1.2749361970 | -3.5531363210 | -1.4617035370 |
| H | 1.5491418190 | -4.1577831930 | -0.5886831910 |
| H | 2.0871174560 | -3.6614442600 | -2.1815420940 |
| H | -0.2106132170 | -3.5534076470 | -3.0045007090 |
| H | 0.0803907410 | -5.1359089970 | -2.2942321360 |
| Cl | -0.2468715190 | 0.0311777190 | -0.2046141150 |
| C | 2.2801566510 | -1.2817700630 | -1.0330210800 |
| C | 3.5759332200 | -1.6680767930 | -1.3327922290 |
| C | -2.4849874860 | -1.9099880180 | -0.1869540570 |
| C | -3.6874134640 | -2.5920988050 | -0.1316565480 |
| H | 2.1102206100 | -0.2517630960 | -0.7502023880 |
| C | 4.6787192240 | -0.8026486970 | -1.3450069830 |
| C | 4.5594489220 | 0.5887792330 | -1.0750018170 |
| C | 6.0003111630 | -1.2610102270 | -1.6581426520 |
| C | 5.6270663760 | 1.4205549930 | -1.1100149910 |
| C | 7.0593993830 | -0.3381412880 | -1.6906039800 |
| O | 6.8573436030 | 0.9736525810 | -1.4090284190 |
| H | 3.5961243700 | 1.0248181700 | -0.8640708190 |
| C | 6.3465557610 | -2.5930062630 | -1.9570833800 |
| C | 8.3573739670 | -0.6789516300 | -1.9994342750 |
| C | 7.6234397890 | -2.9641666750 | -2.2671774620 |
| C | 8.6773225140 | -2.0105812960 | -2.3051718710 |
| H | 5.5831755650 | -3.3591380420 | -1.9436340400 |
| H | 7.8272928650 | -4.0019827690 | -2.4868832350 |
| H | 7.3784929190 | 5.6728360210 | -1.4963803180 |
| C | 6.5755882770 | 5.0479046190 | -1.1242827280 |
| C | 5.5069118290 | 5.6170832190 | -0.4462541990 |
| H | 5.4740004460 | 6.6875825090 | -0.2828237860 |
| C | 4.4821995170 | 4.8079206890 | 0.0279650080 |
| H | 3.6512514400 | 5.2436304810 | 0.5693636680 |

| | | | |
|---|---|---|---|
| C | 4.5208535130 | 3.4409266740 | -0.1788697910 |
| H | 3.7260058410 | 2.8213319170 | 0.2161409660 |
| C | 5.5889767180 | 2.8613632210 | -0.8679757110 |
| C | 6.6211556560 | 3.6796044590 | -1.3325060440 |
| H | 7.4540546790 | 3.2439991830 | -1.8683288980 |
| C | -4.8834715080 | -2.0449583510 | 0.3577577500 |
| C | -4.9448553990 | -0.7508022990 | 0.9432651460 |
| C | -6.1239991250 | -2.7583920930 | 0.2984958210 |
| C | -7.2885347310 | -2.1544774240 | 0.8020004740 |
| C | -6.0976651950 | -0.2391574710 | 1.4369746480 |
| O | -7.2513175550 | -0.9231986110 | 1.3694704060 |
| H | -4.0566381910 | -0.1443516380 | 1.0128039320 |
| C | -8.5307715680 | -2.7476052860 | 0.7650924640 |
| C | -6.2955548780 | -4.0413343710 | -0.2569823960 |
| C | -8.6790109350 | -4.0259659130 | 0.2047262010 |
| C | -7.5123997540 | -4.6585746800 | -0.3060548700 |
| H | -7.5822722270 | -5.6424166540 | -0.7465907400 |
| H | -5.4411482030 | -4.5630497400 | -0.6662848940 |
| H | -6.6823227690 | 4.5166913890 | 3.7869679180 |
| C | -6.5621927040 | 3.5520032530 | 3.3087460570 |
| C | -7.6760702000 | 2.8260520660 | 2.9124459460 |
| H | -8.6706914910 | 3.2227557200 | 3.0766685380 |
| C | -7.5246840560 | 1.5914982080 | 2.3039570440 |
| C | -6.2501412450 | 1.0649641460 | 2.0796262720 |
| C | -5.1336413460 | 1.8016510370 | 2.4854484240 |
| H | -4.1353146880 | 1.4080183070 | 2.3451242300 |
| C | -5.2912899770 | 3.0334971720 | 3.0936054660 |
| H | -4.4165527400 | 3.5897297110 | 3.4081077250 |
| N | -9.8807672780 | -4.6339528300 | 0.1487789420 |
| C | -11.0540612850 | -3.9622337120 | 0.6556828170 |
| C | -10.0155206520 | -5.9481465430 | -0.4391561520 |
| N | 9.9355635080 | -2.3754726200 | -2.6227474240 |
| C | 10.2475884610 | -3.7533948210 | -2.9292058310 |
| C | 10.9889257220 | -1.3878735640 | -2.6429953750 |
| H | -9.7308187160 | -5.9496233070 | -1.4955398790 |
| H | -11.0541332680 | -6.2595081910 | -0.3676159920 |
| H | -9.4027335930 | -6.6875825090 | 0.0839856000 |
| H | -10.9601004030 | -3.7423005090 | 1.7236592660 |
| H | -11.9193906610 | -4.6041530190 | 0.5153592880 |
| H | -11.2364744500 | -3.0209237510 | 0.1276024690 |
| H | 10.0476736530 | -4.4119437080 | -2.0787466800 |
| H | 11.3033886910 | -3.8286223530 | -3.1749858950 |
| H | 9.6728081280 | -4.1139922420 | -3.7869679180 |
| H | 10.7733142750 | -0.5885968340 | -3.3585061880 |
| H | 11.9193906610 | -1.8658389380 | -2.9371863160 |
| H | 11.1329709950 | -0.9340305130 | -1.6572959470 |
| H | -2.4701326330 | -0.8850244470 | 0.1578109550 |
| H | -3.7214053410 | -3.6084303470 | -0.4984341400 |
| H | 3.7576196360 | -2.7050323230 | -1.5771035290 |
| H | 9.1043844480 | 0.1010495810 | -1.9987354240 |
| H | -8.3990497460 | 1.0344283450 | 1.9958396480 |
| H | -9.3689940020 | -2.2037837970 | 1.1751065000 |

Flavylium-9 (Flav-9)

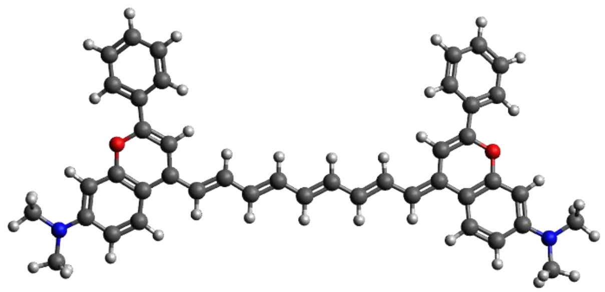

| | | | |
|---|---|---|---|
| 86 | | | |
| C | 1.1084772341 | -1.2939493746 | -0.4092082210 |
| C | -0.0281879978 | -2.0861680222 | -0.3837770330 |
| C | 2.3628424078 | -1.7153460531 | -0.8251008566 |
| C | 3.4627149103 | -0.8739256961 | -0.8681662278 |
| C | 4.7284302333 | -1.2620211668 | -1.2767905054 |
| C | -3.6556726371 | -1.8636579707 | 0.4498852522 |
| C | -4.8418586855 | -2.5787163469 | 0.4169730235 |
| H | 3.2965448455 | 0.1531986895 | -0.5555578329 |
| C | 5.8477246303 | -0.4317217490 | -1.3659580810 |
| C | 5.7862604373 | 0.9622883683 | -1.0948991211 |
| C | 7.1362098270 | -0.9257110081 | -1.7614350494 |
| C | 6.8697315550 | 1.7682683194 | -1.2041651910 |
| C | 8.2124257410 | -0.0316027426 | -1.8662334875 |
| O | 8.0641747518 | 1.2876102793 | -1.5864422933 |
| H | 4.8481860600 | 1.4229623296 | -0.8313757928 |
| C | 7.4291608973 | -2.2670201425 | -2.0631865469 |
| C | 9.4809136670 | -0.4131762153 | -2.2461863999 |
| C | 8.6758711771 | -2.6767158316 | -2.4418936353 |
| C | 9.7482843303 | -1.7540063157 | -2.5500728879 |
| H | 6.6478140815 | -3.0109345981 | -1.9921318962 |
| H | 8.8382196149 | -3.7219536777 | -2.6588463139 |
| H | 8.6914774757 | 5.9740760842 | -1.7195522688 |
| C | 7.9020535179 | 5.3686557979 | -1.2922127159 |
| C | 6.8973214285 | 5.9636027689 | -0.5440938836 |
| H | 6.9020356437 | 7.0341056901 | -0.3813925439 |
| C | 5.8897372769 | 5.1810215281 | 0.0034160752 |
| H | 5.1118424895 | 5.6378490206 | 0.6020788294 |
| C | 5.8826223152 | 3.8145466415 | -0.2023217823 |
| H | 5.1082672326 | 3.2126083965 | 0.2554490899 |
| C | 6.8839221896 | 3.2081164871 | -0.9633696499 |
| C | 7.9003423286 | 4.0004816453 | -1.4991723769 |
| H | 8.6821621717 | 3.5408416021 | -2.0879044083 |
| C | -6.0939564035 | -2.1108459200 | 0.8209320004 |
| C | -6.2805017308 | -0.8242331166 | 1.3956583023 |
| C | -7.2851287272 | -2.8984191571 | 0.6739121786 |

| | | | |
|---|---|---|---|
| C | -8.5162393269 | -2.3673689720 | 1.0873530398 |
| C | -7.4965580288 | -0.3830971794 | 1.7984986758 |
| O | -8.5997214767 | -1.1347555757 | 1.6480053552 |
| H | -5.4430118627 | -0.1564546219 | 1.5168077104 |
| C | -9.7127172320 | -3.0402894603 | 0.9626346587 |
| C | -7.3367867679 | -4.1866483865 | 0.1137424380 |
| C | -9.7410175937 | -4.3214007207 | 0.3968859404 |
| C | -8.5058642703 | -4.8791697906 | -0.0233682678 |
| H | -8.4795500516 | -5.8657826770 | -0.4613434902 |
| H | -6.4246011699 | -4.6552925933 | -0.2283384653 |
| H | -8.5049560397 | 4.3734314922 | 3.9805437346 |
| C | -8.2997735798 | 3.4061822359 | 3.5391621391 |
| C | -9.3211976749 | 2.6826299462 | 2.9421695561 |
| H | -10.3256742998 | 3.0855871498 | 2.9114398380 |
| C | -9.0625639116 | 1.4437424412 | 2.3828180600 |
| C | -7.7708100342 | 0.9155898096 | 2.4064103063 |
| C | -6.7505051992 | 1.6475058785 | 3.0169127987 |
| H | -5.7509095460 | 1.2375179080 | 3.0816992290 |
| C | -7.0144934621 | 2.8828405747 | 3.5772368988 |
| H | -6.2168012156 | 3.4361416783 | 4.0565879584 |
| N | -10.9001594419 | -5.0039368549 | 0.2522663243 |
| C | -12.1416053331 | -4.4136398956 | 0.6898744828 |
| C | -10.9070491614 | -6.3191031473 | -0.3444953586 |
| N | 10.9823152745 | -2.1583390495 | -2.9295614605 |
| C | 11.2408708651 | -3.5485487396 | -3.2218272521 |
| C | 12.0544387481 | -1.1981824019 | -3.0265934435 |
| H | -10.5113329075 | -6.3017168177 | -1.3641761862 |
| H | -11.9301897499 | -6.6821021388 | -0.3901587397 |
| H | -10.3217673683 | -7.0341056901 | 0.2414937953 |
| H | -12.1295194968 | -4.2004935408 | 1.7633951399 |
| H | -12.9563465825 | -5.1050932306 | 0.4932800536 |
| H | -12.3526876331 | -3.4808362571 | 0.1571299822 |
| H | 11.0493069118 | -4.1872449037 | -2.3544125873 |
| H | 12.2854707711 | -3.6640223338 | -3.4978414955 |
| H | 10.6312784321 | -3.9071073894 | -4.0565879584 |
| H | 11.8183720968 | -0.4064588886 | -3.7442624840 |
| H | 12.9563465825 | -1.7007039356 | -3.3650560168 |
| H | 12.2679505241 | -0.7320887665 | -2.0591913868 |
| H | -4.7813643055 | -3.5871001627 | 0.0269545306 |
| H | 4.8457931279 | -2.3027389015 | -1.5521793661 |
| H | 10.2449944415 | 0.3478053204 | -2.2927031491 |
| H | -9.8599977989 | 0.8834782731 | 1.9144640799 |
| H | -10.6081344873 | -2.5487106989 | 1.3114246139 |
| H | 1.0073703227 | -0.2592726607 | -0.0861465027 |
| H | 2.4846684839 | -2.7483060329 | -1.1398739902 |
| C | -2.4336989473 | -2.3684741783 | 0.0350585013 |
| H | -3.6618424612 | -0.8365216182 | 0.8042113837 |
| C | -1.2659642887 | -1.6204345119 | 0.0310533386 |
| H | 0.0519231696 | -3.1180515554 | -0.7149880804 |
| H | -2.3898644329 | -3.3963020902 | -0.3152074801 |
| H | -1.3273807870 | -0.5879117701 | 0.3704616819 |

Indocyanine Green-3 (ICG-3)

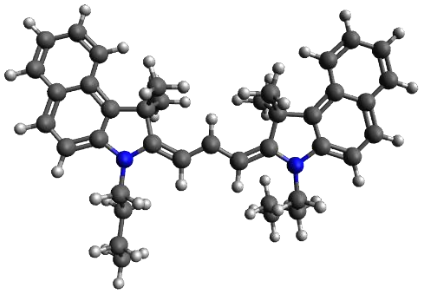

| | | | |
|---|---|---|---|
| 86 | | | |
| C | -2.1137281406 | -1.2783022590 | 1.4341555423 |
| C | -0.7717981384 | -1.0154562151 | 1.2076766758 |
| C | 0.1946054625 | -2.0048647385 | 1.1299707010 |
| C | -3.1334198904 | -0.3367509384 | 1.4754678810 |
| C | -3.0596980911 | 1.1627019014 | 1.2170309420 |
| N | -4.4042459332 | -0.6633681325 | 1.7413905613 |
| C | -4.5095066965 | 1.5667424896 | 1.3568427462 |
| C | -2.5585465984 | 1.4268597756 | -0.2080656150 |
| C | -2.2006984214 | 1.8478996538 | 2.2878295722 |
| C | -5.2486127936 | 0.4522533982 | 1.6584584320 |
| C | -5.1389815554 | 2.8207433417 | 1.2303545668 |
| C | -6.5539644768 | 2.8624530925 | 1.4245816675 |
| C | -7.2641261659 | 1.6793916257 | 1.7273319093 |
| C | -6.6357906256 | 0.4715514341 | 1.8471434595 |
| C | -7.2301720369 | 4.0948979094 | 1.3065650866 |
| C | -6.5526351835 | 5.2438142143 | 1.0104062766 |
| C | -5.1602343720 | 5.2055012523 | 0.8186414376 |
| C | -4.4711958512 | 4.0292243669 | 0.9249584387 |
| H | -8.3034705004 | 4.1133534952 | 1.4557644953 |
| H | -7.0825929690 | 6.1835541611 | 0.9224887685 |
| H | -4.6283747236 | 6.1191892739 | 0.5838063331 |
| H | -3.4014762134 | 4.0326851861 | 0.7713107661 |
| H | -8.3369277320 | 1.7437967303 | 1.8634579941 |
| H | -7.1966724711 | -0.4251923320 | 2.0727650589 |
| H | -2.2500928842 | 2.9296215607 | 2.1762832415 |
| H | -1.1551849386 | 1.5495897382 | 2.2208240906 |
| H | -3.1704040883 | 0.8928230919 | -0.9357494212 |
| H | -1.5253518327 | 1.1069461989 | -0.3373377960 |
| H | -2.6170201552 | 2.4885560279 | -0.4410888166 |
| H | 1.8603247356 | -0.4059133465 | -1.3918240083 |
| C | 1.8034159559 | 0.2416059274 | -0.5162917830 |
| H | 2.4242546420 | 1.1149997474 | -0.7089403480 |
| C | 4.8913027899 | -3.1115426446 | 0.4436738475 |
| C | 6.0618613858 | -2.4388175999 | 0.2319727848 |
| H | 4.8725757362 | -4.1916177519 | 0.4897344936 |

| | | | |
|---|---|---|---|
| H | 6.9855667328 | -2.9913633163 | 0.1092348844 |
| C | 3.7306371625 | -2.3417109289 | 0.5919334373 |
| C | 6.1103350802 | -1.0284438124 | 0.1663897316 |
| C | 7.3339918505 | -0.3619323670 | -0.0531532088 |
| N | 2.4310201732 | -2.8174640303 | 0.8209433587 |
| H | 8.2330343627 | -0.9552760617 | -0.1724678615 |
| C | 3.7184877821 | -0.9726526550 | 0.5367053245 |
| C | 4.9156412391 | -0.2608478705 | 0.3237146569 |
| C | 7.3917414929 | 1.0018230217 | -0.1135736087 |
| C | 1.5512989808 | -1.8104910557 | 0.9099435635 |
| C | 2.2994301958 | -0.4943240478 | 0.7353563471 |
| C | 5.0137819225 | 1.1481373560 | 0.2575727925 |
| C | 6.2181522988 | 1.7598011670 | 0.0449451405 |
| H | 8.3369277320 | 1.5017738112 | -0.2821530757 |
| H | 4.1295399688 | 1.7581855889 | 0.3761682933 |
| H | 6.2699275300 | 2.8405118162 | -0.0022225444 |
| C | 2.1818417193 | 0.3512265821 | 2.0096807807 |
| H | 2.7760162223 | 1.2588994459 | 1.9189591623 |
| H | 2.5498395160 | -0.2031749589 | 2.8734615668 |
| H | 0.7729432779 | 0.5765423170 | -0.4090503092 |
| H | 1.1500349856 | 0.6377109736 | 2.2084513973 |
| H | -2.5610353190 | 1.6001087027 | 3.2866881429 |
| H | -5.0196706069 | -4.7071808578 | 1.6674475660 |
| C | -5.7795299774 | -4.1624849568 | 1.0965695622 |
| H | -6.6514119380 | -4.0826098845 | 1.7540770567 |
| H | -6.5110243889 | -5.9464377735 | 0.1057994657 |
| C | -4.8916351132 | -1.9966868333 | 2.0279305165 |
| C | -6.1471726960 | -4.9504134761 | -0.1483760088 |
| C | -5.2645034572 | -2.7699238046 | 0.7733560362 |
| H | -5.2846640520 | -5.0697111951 | -0.8081415026 |
| H | -4.3906169731 | -2.8365181155 | 0.1173985019 |
| H | -6.9311249775 | -4.4458170395 | -0.7172325555 |
| H | -6.0240527298 | -2.2100659171 | 0.2187872752 |
| H | -4.1288843182 | -2.5246644375 | 2.6021142905 |
| H | -5.7549057724 | -1.8957764362 | 2.6869392868 |
| H | -0.0456018494 | -4.5637870528 | -0.7977754495 |
| C | 0.9038162201 | -4.4105214462 | -1.3220091247 |
| H | 0.9984680379 | -3.3304394595 | -1.4704645101 |
| H | 0.0429099248 | -4.7301212208 | -3.2866881429 |
| C | 2.1458957672 | -4.2374672563 | 0.9083327479 |
| C | 0.8610084265 | -5.1062593510 | -2.6712772278 |
| C | 2.0475153665 | -4.9096742364 | -0.4544283167 |
| H | 0.7225327948 | -6.1835541611 | -2.5565510710 |
| H | 1.9386276223 | -5.9845279519 | -0.2804739963 |
| H | 1.7904532300 | -4.9502806526 | -3.2234514616 |
| H | 2.9934175823 | -4.7810820482 | -0.9892323074 |
| H | 2.9444549282 | -4.6890983421 | 1.4996486354 |
| H | 1.2266916019 | -4.3713364001 | 1.4763563696 |
| H | -0.1526014892 | -3.0251925594 | 1.2338048024 |
| H | -2.3892384543 | -2.3165617801 | 1.5770244035 |
| H | -0.4685240111 | 0.0123753391 | 1.0810990653 |

Indocyanine Green-5 (ICG-5)

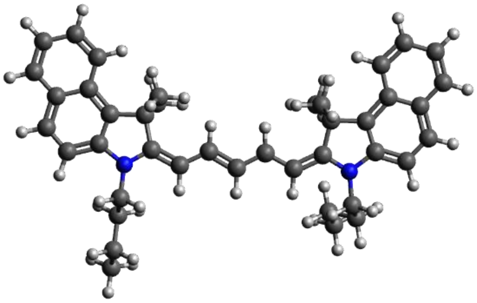

| | | | |
|---|---|---|---|
| 90 | | | |
| C | -3.2602806106 | -0.9916707561 | 1.6243757130 |
| C | -1.9105992201 | -0.7628576887 | 1.4018074663 |
| C | -0.9473119441 | -1.7568134322 | 1.3415331193 |
| C | 0.3910895042 | -1.4777883232 | 1.1131137597 |
| C | 1.3818214999 | -2.4417735840 | 1.0073598032 |
| H | -1.5633409382 | 0.2541553659 | 1.2590962999 |
| C | -4.2612527153 | -0.0318628205 | 1.6523654852 |
| H | -3.5560917512 | -2.0231816798 | 1.7754145417 |
| C | -4.1553648769 | 1.4645615379 | 1.3892310398 |
| N | -5.5421273049 | -0.3319110833 | 1.9111194013 |
| C | -5.5981285456 | 1.8979862804 | 1.5149852504 |
| C | -3.6333368126 | 1.7154571719 | -0.0310642920 |
| C | -3.2922572043 | 2.1330558104 | 2.4678689017 |
| C | -6.3617133239 | 0.7993449892 | 1.8160214871 |
| C | -6.2023134946 | 3.1633485681 | 1.3792412317 |
| C | -7.6177499209 | 3.2341085623 | 1.5614173789 |
| C | -8.3536359744 | 2.0665863853 | 1.8630886283 |
| C | -7.7499632690 | 0.8474477303 | 1.9935424621 |
| C | -8.2681071724 | 4.4792658042 | 1.4330231030 |
| C | -7.5653650775 | 5.6135482414 | 1.1387481640 |
| C | -6.1723451286 | 5.5468703205 | 0.9597327925 |
| C | -5.5079588591 | 4.3574248594 | 1.0761427912 |
| H | -9.3421205544 | 4.5196589620 | 1.5728698330 |
| H | -8.0758755990 | 6.5632536542 | 1.0428580714 |
| H | -5.6201454942 | 6.4489503101 | 0.7268694024 |
| H | -4.4369771336 | 4.3385094186 | 0.9329389608 |
| H | -9.4261168591 | 2.1526390729 | 1.9898043540 |
| H | -8.3300018601 | -0.0372625452 | 2.2183718832 |
| H | -3.3018252581 | 3.2145057203 | 2.3427232449 |
| H | -2.2580940442 | 1.7946167966 | 2.4237953162 |
| H | -4.2516253936 | 1.1962940731 | -0.7641525855 |
| H | -2.6071716375 | 1.3702748524 | -0.1497571615 |
| H | -3.6641809669 | 2.7783408980 | -0.2643721910 |
| H | 2.9973784740 | -0.7872559350 | -1.5169283893 |
| C | 2.9191316801 | -0.1507578356 | -0.6348581790 |

| | | | |
|---|---|---|---|
| H | 3.5071910108 | 0.7466235891 | -0.8208930868 |
| C | 6.0966786029 | -3.4355097190 | 0.2756119158 |
| C | 7.2496108340 | -2.7343461598 | 0.0599854162 |
| H | 6.1037071352 | -4.5159981138 | 0.3154362080 |
| H | 8.1851893309 | -3.2642822490 | -0.0725004582 |
| C | 4.9187845519 | -2.6945366846 | 0.4371374501 |
| C | 7.2642341180 | -1.3228965549 | 0.0019590142 |
| C | 8.4696681406 | -0.6261431589 | -0.2240435929 |
| N | 3.6341115281 | -3.2024621752 | 0.6723038195 |
| H | 9.3816712619 | -1.1972608800 | -0.3533877419 |
| C | 4.8743987518 | -1.3252804984 | 0.3919689968 |
| C | 6.0528791312 | -0.5849848109 | 0.1730065639 |
| C | 8.4944309900 | 0.7388997180 | -0.2788557723 |
| C | 2.7307810927 | -2.2155095635 | 0.7783980370 |
| C | 3.4465499439 | -0.8814643023 | 0.6072986279 |
| C | 6.1169381539 | 0.8263441417 | 0.1121358341 |
| C | 7.3043526328 | 1.4678112154 | -0.1077267293 |
| H | 9.4261168591 | 1.2618813597 | -0.4528016258 |
| H | 5.2189513504 | 1.4139880682 | 0.2395098563 |
| H | 7.3294832604 | 2.5496479538 | -0.1510102532 |
| C | 3.3209867663 | -0.0459325852 | 1.8877514632 |
| H | 3.8994748681 | 0.8721650705 | 1.7997328822 |
| H | 3.7035491083 | -0.5997636731 | 2.7456266312 |
| H | 1.8769625975 | 0.1427947764 | -0.5203563934 |
| H | 2.2855572851 | 0.2214998378 | 2.0928965490 |
| H | -3.6802774805 | 1.9097594158 | 3.4622051237 |
| H | -6.2535288563 | -4.3619345079 | 1.8531586173 |
| C | -6.9996375559 | -3.7998038040 | 1.2811698705 |
| H | -7.8680237716 | -3.6936683107 | 1.9397267234 |
| H | -7.7809518887 | -5.5681014409 | 0.3003414270 |
| C | -6.0591504108 | -1.6523697186 | 2.2024611108 |
| C | -7.3906164621 | -4.5834973178 | 0.0406916137 |
| C | -6.4482248081 | -2.4229443992 | 0.9510638108 |
| H | -6.5329323270 | -4.7294385821 | -0.6199020425 |
| H | -5.5744674433 | -2.5153323967 | 0.2982845150 |
| H | -8.1616446475 | -4.0606283908 | -0.5294767633 |
| H | -7.1921501224 | -1.8472635827 | 0.3914202400 |
| H | -5.3091829507 | -2.1951293601 | 2.7796310321 |
| H | -6.9209160900 | -1.5295810173 | 2.8599188627 |
| H | 1.2020023081 | -4.9602053719 | -0.9729294147 |
| C | 2.1521030163 | -4.7961805335 | -1.4922385664 |
| H | 2.2382382555 | -3.7145634036 | -1.6341046367 |
| H | 1.3019829408 | -5.1105800832 | -3.4622051237 |
| C | 3.3813854700 | -4.6289451766 | 0.7457821973 |
| C | 2.1203994781 | -5.4842855857 | -2.8457168037 |
| C | 3.2970594878 | -5.2900987024 | -0.6234126043 |
| H | 1.9892741184 | -6.5632536542 | -2.7378323795 |
| H | 3.1995924470 | -6.3676448717 | -0.4591554571 |
| H | 3.0509994755 | -5.3183816388 | -3.3931845351 |
| H | 4.2437036102 | -5.1463053685 | -1.1531227348 |
| H | 4.1896851966 | -5.0694159142 | 1.3325561564 |
| H | 2.4653611307 | -4.7882598084 | 1.3122278124 |
| H | 1.0572559260 | -3.4707407527 | 1.0974998558 |

| | | | |
|---|---|---|---|
| H | -1.2522513922 | -2.7918380929 | 1.4696257642 |
| H | 0.6528131631 | -0.4313419009 | 1.0061183534 |

Indocyanine Green-7 (ICG-7)

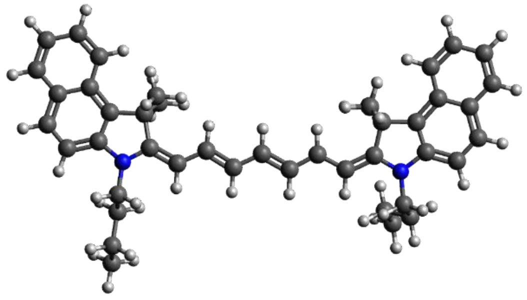

| | | | |
|---|---|---|---|
| 94 | | | |
| C | -4.4079253026 | -0.6855798184 | 1.8037070033 |
| C | -3.0541840642 | -0.4732559140 | 1.5793279121 |
| C | -2.1052067993 | -1.4802987401 | 1.5350124926 |
| C | -0.7602054524 | -1.2305789379 | 1.3080737710 |
| C | 0.2305228391 | -2.1967274754 | 1.2249590755 |
| C | 1.5602341386 | -1.8850531884 | 0.9951241669 |
| C | 2.5706716367 | -2.8291710186 | 0.8750041064 |
| H | -2.6936312623 | 0.5371789382 | 1.4239418922 |
| C | -5.3998754643 | 0.2813984690 | 1.8249074315 |
| H | -4.7125281939 | -1.7131235002 | 1.9648192502 |
| C | -5.2818504166 | 1.7754796305 | 1.5527267010 |
| N | -6.6849072703 | -0.0062622836 | 2.0870957080 |
| C | -6.7210093298 | 2.2216924704 | 1.6774564245 |
| C | -4.7583586479 | 2.0142586931 | 0.1309115721 |
| C | -4.4112443023 | 2.4422736565 | 2.6264305143 |
| C | -7.4936012340 | 1.1308967612 | 1.9853444482 |
| C | -7.3150854058 | 3.4909616737 | 1.5347251493 |
| C | -8.7299296828 | 3.5748076921 | 1.7164223912 |
| C | -9.4754801004 | 2.4151734313 | 2.0247099437 |
| C | -8.8815675402 | 1.1920760013 | 2.1623955138 |
| C | -9.3698542048 | 4.8246164021 | 1.5809043311 |
| C | -8.6577694856 | 5.9514522571 | 1.2804544228 |
| C | -7.2652760681 | 5.8720513276 | 1.1021333318 |
| C | -6.6108886026 | 4.6777660113 | 1.2252024971 |
| H | -10.4435506096 | 4.8745696761 | 1.7204113293 |
| H | -9.1603180062 | 6.9048603231 | 1.1791698974 |
| H | -6.7054451686 | 6.7681997693 | 0.8645226926 |
| H | -5.5400513425 | 4.6487919694 | 1.0825929327 |
| H | -10.5472698796 | 2.5108671991 | 2.1506033280 |
| H | -9.4685912710 | 0.3132210720 | 2.3921441666 |
| H | -4.4082052373 | 3.5229255671 | 2.4936424796 |

| | | | |
|---|---|---|---|
| H | -3.3812240709 | 2.0913079589 | 2.5843614521 |
| H | -5.3836704694 | 1.4994443730 | -0.5992942928 |
| H | -3.7366745458 | 1.6559882326 | 0.0129002830 |
| H | -4.7762591267 | 3.0765126982 | -0.1068059609 |
| H | 4.1586092627 | -1.1207455540 | -1.6325197508 |
| C | 4.0642617218 | -0.4953183719 | -0.7440962386 |
| H | 4.6321715703 | 0.4170699904 | -0.9195692976 |
| C | 7.3034350395 | -3.7283431792 | 0.1406627213 |
| C | 8.4436892420 | -3.0039905438 | -0.0656100412 |
| H | 7.3307268269 | -4.8088956044 | 0.1704204747 |
| H | 9.3893469779 | -3.5151228486 | -0.2006312038 |
| C | 6.1109669178 | -3.0117255276 | 0.3064767080 |
| C | 8.4318409633 | -1.5920720878 | -0.1111457435 |
| C | 9.6242090705 | -0.8703547551 | -0.3281729752 |
| N | 4.8370965184 | -3.5461432189 | 0.5348780755 |
| H | 10.5472698796 | -1.4229205802 | -0.4599322893 |
| C | 6.0412393485 | -1.6428609326 | 0.2734825065 |
| C | 7.2061061140 | -0.8791163428 | 0.0632837780 |
| C | 9.6229909045 | 0.4953210178 | -0.3718152813 |
| C | 3.9137674164 | -2.5761216332 | 0.6495539604 |
| C | 4.6050729326 | -1.2273864116 | 0.4914664907 |
| C | 7.2433903554 | 0.5337847953 | 0.0139538749 |
| C | 8.4186289950 | 1.1997882305 | -0.1979006492 |
| H | 10.5449182159 | 1.0374747513 | -0.5390606925 |
| H | 6.3337166723 | 1.1025699030 | 0.1435366829 |
| H | 8.4229010429 | 2.2822409313 | -0.2325300084 |
| C | 4.4629814327 | -0.4058180946 | 1.7791632334 |
| H | 5.0282242280 | 0.5216158353 | 1.7031114667 |
| H | 4.8500894073 | -0.9626808389 | 2.6330732763 |
| H | 3.0154345310 | -0.2269069710 | -0.6289292771 |
| H | 3.4230719369 | -0.1553198727 | 1.9827795261 |
| H | -4.8016458761 | 2.2301714775 | 3.6223045253 |
| H | -7.4332406311 | -4.0307044757 | 2.0599261605 |
| C | -8.1755508965 | -3.4650600349 | 1.4864869388 |
| H | -9.0403577573 | -3.3448447226 | 2.1474351438 |
| H | -8.9809861867 | -5.2318638045 | 0.5225609459 |
| C | -7.2124456574 | -1.3196262395 | 2.3886976352 |
| C | -8.5796094767 | -4.2541400439 | 0.2536780480 |
| C | -7.6109261803 | -2.0966685244 | 1.1442262069 |
| H | -7.7259132214 | -4.4159296376 | -0.4083660831 |
| H | -6.7390066480 | -2.2029532457 | 0.4911696223 |
| H | -9.3460528705 | -3.7266783875 | -0.3185165488 |
| H | -8.3499428464 | -1.5181608431 | 0.5809355465 |
| H | -6.4659257870 | -1.8646793352 | 2.9682985967 |
| H | -8.0718766066 | -1.1851114995 | 3.0471131978 |
| H | 2.4396611085 | -5.3228642993 | -1.1327885698 |
| C | 3.3889262458 | -5.1436229690 | -1.6484289356 |
| H | 3.4617076971 | -4.0601944654 | -1.7833400294 |
| H | 2.5474497515 | -5.4558698257 | -3.6223045253 |
| C | 4.6102694532 | -4.9771236977 | 0.5946571126 |
| C | 3.3687354878 | -5.8237861291 | -3.0061231281 |
| C | 4.5381103143 | -5.6282741859 | -0.7799892730 |
| H | 3.2497452208 | -6.9048603231 | -2.9050042351 |

| | | | |
|---|---|---|---|
| H | 4.4549691600 | -6.7084122654 | -0.6244699005 |
| H | 4.2986994141 | -5.6440066255 | -3.5503787536 |
| H | 5.4840696813 | -5.4675979811 | -1.3062385843 |
| H | 5.4259998867 | -5.4090847360 | 1.1776246998 |
| H | 3.6971841644 | -5.1579007004 | 1.1596088604 |
| H | 2.2647299269 | -3.8649412900 | 0.9527582363 |
| H | 1.7999535491 | -0.8322793937 | 0.9007866803 |
| H | -0.0493500119 | -3.2404100049 | 1.3393280377 |
| H | -2.4263618258 | -2.5084774346 | 1.6777797518 |
| H | -0.4589702450 | -0.1920648825 | 1.1793392341 |

Indocyanine Green-9 (ICG-9)

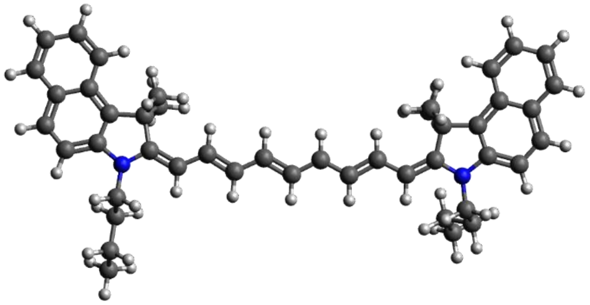

| | | | |
|---|---|---|---|
| 98 | | | |
| C | -5.5661540687 | -0.4342841264 | 1.9746524219 |
| C | -4.2111428049 | -0.2179284206 | 1.7513655525 |
| C | -3.2595942678 | -1.2209177489 | 1.7165282266 |
| C | -1.9130477232 | -0.9699861308 | 1.4908605888 |
| C | -0.9228914724 | -1.9362854838 | 1.4234846831 |
| C | 0.4095736655 | -1.6339966845 | 1.1932438955 |
| C | 1.4328701708 | -2.5659968849 | 1.0930055534 |
| C | 2.7497378093 | -2.2101706942 | 0.8613576835 |
| C | 3.7893710746 | -3.1228141200 | 0.7296375286 |
| H | -3.8542566721 | 0.7928329340 | 1.5900172925 |
| H | -3.5775308383 | -2.2490837432 | 1.8670500492 |
| H | -1.6125951690 | 0.0671150213 | 1.3509244279 |
| H | -1.2040798580 | -2.9779957698 | 1.5514328626 |
| H | 0.6732584553 | -0.5840524005 | 1.0772651762 |
| H | 1.1870324129 | -3.6194300345 | 1.1965782413 |
| H | 2.9563026776 | -1.1496978997 | 0.7751912229 |
| C | -6.5606612149 | 0.5279156904 | 1.9916226071 |
| H | -5.8664642742 | -1.4625136219 | 2.1395456402 |
| C | -6.4470923688 | 2.0226853116 | 1.7204743014 |
| N | -7.8470911072 | 0.2359929443 | 2.2507368929 |
| C | -7.8881854248 | 2.4641609567 | 1.8427126584 |
| C | -5.9220654569 | 2.2640763930 | 0.2997117060 |
| C | -5.5803603611 | 2.6916881234 | 2.7957682923 |

| | | | |
|---|---|---|---|
| C | -8.6580150238 | 1.3704605936 | 2.1482691271 |
| C | -8.4858900692 | 3.7315711604 | 1.6997723582 |
| C | -9.9013545419 | 3.8115774687 | 1.8784982698 |
| C | -10.6440066558 | 2.6495693187 | 2.1841145356 |
| C | -10.0466936025 | 1.4281567890 | 2.3219858469 |
| C | -10.5444345479 | 5.0597028658 | 1.7427140336 |
| C | -9.8350025942 | 6.1888665715 | 1.4446739985 |
| C | -8.4419493072 | 6.1133371027 | 1.2690839913 |
| C | -7.7845397105 | 4.9207684374 | 1.3925960779 |
| H | -11.6185664656 | 5.1064535590 | 1.8801582989 |
| H | -10.3400779362 | 7.1409326440 | 1.3432100820 |
| H | -7.8839440692 | 7.0111127645 | 1.0332635587 |
| H | -6.7133542517 | 4.8948096475 | 1.2521455567 |
| H | -11.7164018137 | 2.7418043840 | 2.3076366766 |
| H | -10.6319075471 | 0.5475169449 | 2.5495627563 |
| H | -5.5773461675 | 3.7722267901 | 2.6619912254 |
| H | -4.5501215795 | 2.3409843685 | 2.7572801726 |
| H | -6.5435201054 | 1.7459240228 | -0.4314313318 |
| H | -4.8984530328 | 1.9107436855 | 0.1835483039 |
| H | -5.9446962511 | 3.3262049832 | 0.0615644811 |
| H | 5.3161511567 | -1.3612740765 | -1.7764321496 |
| C | 5.2033120460 | -0.7419038572 | -0.8858813448 |
| H | 5.7384144927 | 0.1901767781 | -1.0609564625 |
| C | 8.5445795304 | -3.8763508806 | -0.0187296996 |
| C | 9.6623616918 | -3.1174831884 | -0.2241097400 |
| H | 8.6050687233 | -4.9556713812 | 0.0083493586 |
| H | 10.6228697289 | -3.5996192258 | -0.3611211383 |
| C | 7.3306823760 | -3.1972508377 | 0.1504503837 |
| C | 9.6075352245 | -1.7066558959 | -0.2668275734 |
| C | 10.7769042301 | -0.9483147350 | -0.4841670197 |
| N | 6.0753490556 | -3.7711446226 | 0.3798979346 |
| H | 11.7164018137 | -1.4721377686 | -0.6173641084 |
| C | 7.2197117902 | -1.8308146371 | 0.1214996255 |
| C | 8.3606655650 | -1.0321459364 | -0.0895791247 |
| C | 10.7336672738 | 0.4167350212 | -0.5268695070 |
| C | 5.1221770026 | -2.8289503517 | 0.5021564003 |
| C | 5.7723321084 | -1.4592136726 | 0.3456167740 |
| C | 8.3544953583 | 0.3813092503 | -0.1377940514 |
| C | 9.5082367013 | 1.0834480831 | -0.3511757810 |
| H | 11.6383322942 | 0.9870685016 | -0.6946832546 |
| H | 7.4277837553 | 0.9214288265 | -0.0065311056 |
| H | 9.4787504158 | 2.1655382975 | -0.3853082428 |
| C | 5.6106012533 | -0.6443923655 | 1.6351677538 |
| H | 6.1511854471 | 0.2978267767 | 1.5611056935 |
| H | 6.0130754769 | -1.1931888610 | 2.4872076843 |
| H | 4.1460640576 | -0.5106396408 | -0.7667815380 |
| H | 4.5647866686 | -0.4216838869 | 1.8406779718 |
| H | -5.9737337943 | 2.4801463431 | 3.7905945324 |
| H | 3.5142634647 | -4.1676978819 | 0.8008504985 |
| H | -8.5718305712 | -3.7921926477 | 2.2190455258 |
| C | -9.3158712461 | -3.2311134190 | 1.6433805847 |
| H | -10.1837393973 | -3.1170021662 | 2.3014516529 |
| H | -10.1049147418 | -5.0032422992 | 0.6752010650 |

| | | | |
|---|---|---|---|
| C | -8.3702579610 | -1.0791294676 | 2.5501210382 |
| C | -9.7105348135 | -4.0220005683 | 0.4086952313 |
| C | -8.7589666968 | -1.8588509769 | 1.3039969895 |
| H | -8.8537418129 | -4.1760625867 | -0.2511887982 |
| H | -7.8840641924 | -1.9590713269 | 0.6540540838 |
| H | -10.4794801573 | -3.4997243198 | -0.1649165021 |
| H | -9.4997243561 | -1.2849556045 | 0.7382811098 |
| H | -7.6244498340 | -1.6210016788 | 3.1337358092 |
| H | -9.2339159780 | -0.9487153221 | 3.2038592032 |
| H | 3.7286352850 | -5.6105160558 | -1.3013071815 |
| C | 4.6713365077 | -5.3924945000 | -1.8140465976 |
| H | 4.7077931159 | -4.3056311069 | -1.9345947625 |
| H | 3.8380246892 | -5.7087837418 | -3.7905945324 |
| C | 5.8910016940 | -5.2082138149 | 0.4283292948 |
| C | 4.6732584795 | -6.0550328826 | -3.1805881045 |
| C | 5.8361408303 | -5.8498909719 | -0.9514913860 |
| H | 4.5932389418 | -7.1409326440 | -3.0936215278 |
| H | 5.7857441058 | -6.9333877394 | -0.8052035106 |
| H | 5.5951471610 | -5.8348358792 | -3.7237599750 |
| H | 6.7757341950 | -5.6563787896 | -1.4781497513 |
| H | 6.7191360423 | -5.6215340553 | 1.0074767514 |
| H | 4.9839294463 | -5.4204313545 | 0.9920189548 |

Indocyanine Green-11 (ICG-11)

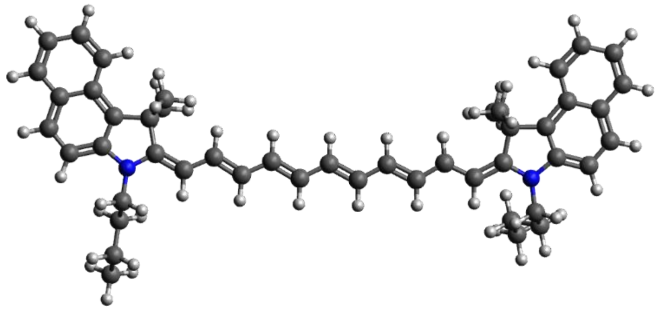

| | | | |
|---|---|---|---|
| 102 | | | |
| C | -6.7496113601 | -0.0192594060 | 2.1259743605 |
| C | -5.3882219229 | 0.1560517248 | 1.8963961027 |
| C | -4.4691024260 | -0.8754438527 | 1.8734165807 |
| C | -3.1136207236 | -0.6731658493 | 1.6440902114 |
| C | -2.1589987250 | -1.6738400271 | 1.5941528127 |
| C | 1.5046530646 | -2.1055407102 | 1.0599018123 |
| C | 2.5201426179 | -3.0478498125 | 0.9562338725 |
| C | 3.8402699883 | -2.7059489211 | 0.7302497867 |
| C | 4.8711681247 | -3.6309327603 | 0.5995371852 |
| H | -5.0012441259 | 1.1535429016 | 1.7218956715 |
| H | -4.8200818823 | -1.8905968493 | 2.0388596142 |

| | | | |
|---|---|---|---|
| H | -2.7772365050 | 0.3505174845 | 1.4886957247 |
| C | -7.7188127211 | 0.9663670876 | 2.1370447485 |
| H | -7.0758470174 | -1.0376821888 | 2.3030460640 |
| C | -7.5696598800 | 2.4558105398 | 1.8521457720 |
| N | -9.0126018814 | 0.7086037913 | 2.4032801726 |
| C | -8.9996248677 | 2.9331871570 | 1.9733194244 |
| C | -7.0416161287 | 2.6730325087 | 0.4286637348 |
| C | -6.6833324388 | 3.1120861096 | 2.9192703246 |
| C | -9.7951126840 | 1.8609354061 | 2.2898176911 |
| C | -9.5676908236 | 4.2128303511 | 1.8186864237 |
| C | -10.9810174202 | 4.3277628870 | 1.9958020490 |
| C | -11.7509057579 | 3.1866508882 | 2.3122733277 |
| C | -11.1820380985 | 1.9531646505 | 2.4628015004 |
| C | -11.5947688355 | 5.5891494660 | 1.8473344925 |
| C | -10.8591590125 | 6.6987410220 | 1.5392099265 |
| C | -9.4681208324 | 6.5890865000 | 1.3659652328 |
| C | -8.8387840888 | 5.3826645035 | 1.5013293023 |
| H | -12.6676508365 | 5.6619510261 | 1.9834245931 |
| H | -11.3418760866 | 7.6612858623 | 1.4281091631 |
| H | -8.8890342312 | 7.4713154634 | 1.1223262065 |
| H | -7.7683130193 | 5.3301431323 | 1.3625806152 |
| H | -12.8209016262 | 3.3053035402 | 2.4341460232 |
| H | -11.7873052149 | 1.0883080470 | 2.6983705737 |
| H | -6.6489766643 | 4.1905837396 | 2.7732491545 |
| H | -5.6637571080 | 2.7311007158 | 2.8837334264 |
| H | -7.6813432676 | 2.1710147528 | -0.2979352580 |
| H | -6.0300599499 | 2.2867627509 | 0.3117012750 |
| H | -7.0309600864 | 3.7341831793 | 0.1853115225 |
| H | 6.4260591606 | -1.8771351092 | -1.8931517170 |
| C | 6.3178471758 | -1.2608955025 | -0.9998465446 |
| H | 6.8639194668 | -0.3339711703 | -1.1686270990 |
| C | 9.6185034814 | -4.4405178585 | -0.1371712098 |
| C | 10.7460590174 | -3.6946340592 | -0.3367927434 |
| H | 9.6657695933 | -5.5206210123 | -0.1138657146 |
| H | 11.7011017119 | -4.1877854503 | -0.4729558705 |
| C | 8.4120650804 | -3.7479047453 | 0.0314437121 |
| C | 10.7085144208 | -2.2831590538 | -0.3741447195 |
| C | 11.8875652533 | -1.5381552763 | -0.5852208239 |
| N | 7.1503435322 | -4.3075435535 | 0.2559619770 |
| H | 12.8209016262 | -2.0730127138 | -0.7180866476 |
| C | 8.3181715736 | -2.3798746629 | 0.0071465387 |
| C | 9.4692569760 | -1.5945168867 | -0.1976175394 |
| C | 11.8611794173 | -0.1724810909 | -0.6221833256 |
| C | 6.2070533352 | -3.3532612867 | 0.3785929835 |
| C | 6.8748517396 | -1.9911590478 | 0.2294195045 |
| C | 9.4806491038 | -0.1808024031 | -0.2399702405 |
| C | 10.6434076271 | 0.5082160090 | -0.4469642716 |
| H | 12.7731761884 | 0.3875244371 | -0.7851180589 |
| H | 8.5600897155 | 0.3698726716 | -0.1092539348 |
| H | 10.6270613419 | 1.5907380320 | -0.4765299337 |
| C | 6.7206219721 | -1.1798297814 | 1.5221651273 |
| H | 7.2700815267 | -0.2423975766 | 1.4521634441 |
| H | 7.1175292510 | -1.7360501045 | 2.3719930969 |

| | | | |
|---|---|---|---|
| H | 5.2629000501 | -1.0185905320 | -0.8821876876 |
| H | 5.6769346799 | -0.9481141768 | 1.7283182957 |
| H | -7.0815743028 | 2.9228443877 | 3.9166286778 |
| H | -9.8407738013 | -3.2990714197 | 2.4173150116 |
| C | -10.5724613625 | -2.7251331839 | 1.8384802987 |
| H | -11.4341217354 | -2.5813102161 | 2.4989887574 |
| H | -11.4129646998 | -4.4864816652 | 0.8943106092 |
| C | -9.5673336289 | -0.5893425855 | 2.7178427090 |
| C | -10.9935610377 | -3.5193007030 | 0.6147346266 |
| C | -9.9816603645 | -1.3716602384 | 1.4817640319 |
| H | -10.1443733726 | -3.7040703479 | -0.0471126505 |
| H | -9.1124454572 | -1.5012795597 | 0.8293747398 |
| H | -11.7508676571 | -2.9832711378 | 0.0382611026 |
| H | -10.7097960881 | -0.7846555580 | 0.9130159666 |
| H | -8.8326705040 | -1.1442309695 | 3.3034699410 |
| H | -10.4241567926 | -0.4309693601 | 3.3745527333 |
| H | 4.7839078547 | -6.1091624234 | -1.4267814574 |
| C | 5.7296560800 | -5.9094059496 | -1.9412983799 |
| H | 5.7840697890 | -4.8237501390 | -2.0659429058 |
| H | 4.8905381287 | -6.2188973804 | -3.9166286778 |
| C | 6.9482644994 | -5.7418668450 | 0.3024618402 |
| C | 5.7195620240 | -6.5772763221 | -3.3051421411 |
| C | 6.8876001487 | -6.3820501347 | -1.0777922367 |
| H | 5.6205381437 | -7.6612858623 | -3.2137934477 |
| H | 6.8240761242 | -7.4651182686 | -0.9331183519 |
| H | 6.6451390709 | -6.3756423274 | -3.8493210359 |
| H | 7.8301817774 | -6.1991230849 | -1.6030043606 |
| H | 7.7697391520 | -6.1666659984 | 0.8829465277 |
| H | 6.0373112657 | -5.9429552580 | 0.8641146970 |
| C | -0.8140365372 | -1.4249166367 | 1.3643226667 |
| C | 0.1710295577 | -2.3978804480 | 1.2881692979 |
| H | -2.4778946939 | -2.7025833538 | 1.7384181727 |
| H | 4.5825839579 | -4.6725467361 | 0.6664865740 |
| H | 4.0595658029 | -1.6476711538 | 0.6487908868 |
| H | 2.2623094702 | -4.0990514216 | 1.0540909169 |
| H | -0.5093172268 | -0.3884563182 | 1.2307577998 |
| H | -0.1185081866 | -3.4381825933 | 1.4097144327 |
| H | 1.7784583693 | -1.0576448713 | 0.9496995918 |

IR-27

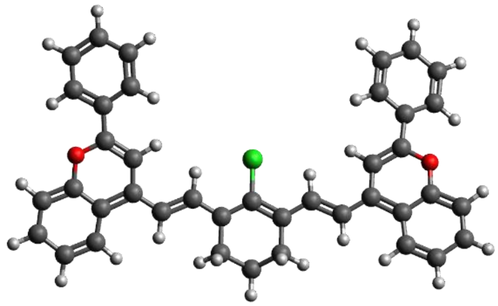

| 73 | | | |
|---|---|---|---|
| C | -0.1860076176 | -2.1065943433 | -1.1605093142 |
| C | -1.3596841540 | -2.8747009931 | -1.1944665336 |
| C | 1.0824700297 | -2.5828177506 | -1.5262474731 |
| C | -1.2778839057 | -4.2736093745 | -1.7447593413 |
| C | -0.0961218278 | -4.4628832709 | -2.6722739913 |
| H | -2.2018370495 | -4.5048757256 | -2.2779458218 |
| H | -1.2154905060 | -4.9843941603 | -0.9120098567 |
| C | 1.1829291360 | -4.0069023243 | -2.0006940191 |
| H | 1.4110365509 | -4.6605679565 | -1.1499792553 |
| H | 2.0163573238 | -4.0990855917 | -2.6979010554 |
| H | -0.2515876518 | -3.8798558576 | -3.5846300649 |
| H | -0.0156098017 | -5.5094121010 | -2.9706437129 |
| Cl | -0.3070284097 | -0.4670644550 | -0.6013209057 |
| C | 2.2138169747 | -1.7783511241 | -1.4443711789 |
| C | 3.5147845217 | -2.1804454873 | -1.7043955438 |
| C | -2.5646256718 | -2.3802500755 | -0.7048784702 |
| C | -3.7696751767 | -3.0631994485 | -0.6784358721 |
| H | 2.0490665199 | -0.7554694652 | -1.1340241479 |
| C | 4.6276795122 | -1.3370123072 | -1.6639578532 |
| C | 4.5298701451 | 0.0543290306 | -1.4331734518 |
| C | 5.9690450373 | -1.8372839745 | -1.8910368527 |
| C | 5.6165979063 | 0.8726325446 | -1.4330344692 |
| C | 7.0333314752 | -0.9286509439 | -1.8836029559 |
| O | 6.8454142279 | 0.3939197479 | -1.6559785450 |
| H | 3.5656804207 | 0.5174407591 | -1.2992210378 |
| C | 6.2854694791 | -3.1843567736 | -2.1239018113 |
| C | 8.3470662235 | -1.3207754273 | -2.1011524364 |
| C | 7.5823925562 | -3.5859668692 | -2.3393930632 |
| C | 8.6183321547 | -2.6504758384 | -2.3303583512 |
| H | 5.4994607445 | -3.9261581599 | -2.1297132872 |
| H | 7.8005429327 | -4.6313074271 | -2.5143592593 |
| H | 7.4117590109 | 5.0915861671 | -1.9017565984 |
| C | 6.5951962233 | 4.4833756186 | -1.5339354544 |
| C | 5.5112097325 | 5.0798969163 | -0.9067410997 |
| H | 5.4819066619 | 6.1548501684 | -0.7799882570 |
| C | 4.4669658078 | 4.2958815247 | -0.4351969603 |
| H | 3.6270308100 | 4.7562929649 | 0.0692620802 |

| | | | |
|---|---|---|---|
| C | 4.5010818227 | 2.9243205350 | -0.5976925818 |
| H | 3.6946398341 | 2.3218212474 | -0.1998598925 |
| C | 5.5843926415 | 2.3163604260 | -1.2360330011 |
| C | 6.6373635325 | 3.1103456721 | -1.6946312398 |
| H | 7.4809905333 | 2.6485919558 | -2.1890667615 |
| C | -4.9588164748 | -2.5547766328 | -0.1479680836 |
| C | -5.0410073109 | -1.2977562222 | 0.4933834395 |
| C | -6.2003505507 | -3.2988889372 | -0.2211571162 |
| C | -7.3506262389 | -2.7383836574 | 0.3450184561 |
| C | -6.1962336115 | -0.8288990068 | 1.0390443201 |
| O | -7.3295768713 | -1.5356500686 | 0.9675813494 |
| H | -4.1685003834 | -0.6694789867 | 0.5672629717 |
| C | -8.5830711135 | -3.3762560274 | 0.3103978945 |
| C | -6.3426521170 | -4.5493901512 | -0.8416842561 |
| C | -8.6832545322 | -4.6035543870 | -0.3042674311 |
| C | -7.5575106387 | -5.1913825048 | -0.8836079363 |
| H | -7.6409623375 | -6.1548501684 | -1.3691303827 |
| H | -5.4854539143 | -5.0195853327 | -1.3021960315 |
| H | -6.8034356995 | 3.8105823180 | 3.5846300649 |
| C | -6.6781894493 | 2.8680754738 | 3.0665408366 |
| C | -7.7888078600 | 2.1617412983 | 2.6294095271 |
| H | -8.7835966263 | 2.5527152069 | 2.8010928531 |
| C | -7.6318623531 | 0.9556178975 | 1.9715786371 |
| C | -6.3546969691 | 0.4411604847 | 1.7366237761 |
| C | -5.2422238192 | 1.1578220050 | 2.1848474842 |
| H | -4.2438122889 | 0.7647327728 | 2.0445149796 |
| C | -5.4050064077 | 2.3605544222 | 2.8443249431 |
| H | -4.5356545763 | 2.9018544208 | 3.1952049099 |
| H | -2.5400734408 | -1.3746271336 | -0.3083021160 |
| H | -3.7991680240 | -4.0600239174 | -1.0931484710 |
| H | 3.6880179048 | -3.2180105384 | -1.9488843664 |
| H | 9.1280730028 | -0.5722954854 | -2.0821779035 |
| H | -8.5005728397 | 0.4100372978 | 1.6306251957 |
| H | -9.4367721695 | -2.8942788389 | 0.7680233096 |
| H | 9.6388648429 | -2.9688107117 | -2.5001095961 |
| H | -9.6388648429 | -5.1108024303 | -0.3384649700 |

IR-26

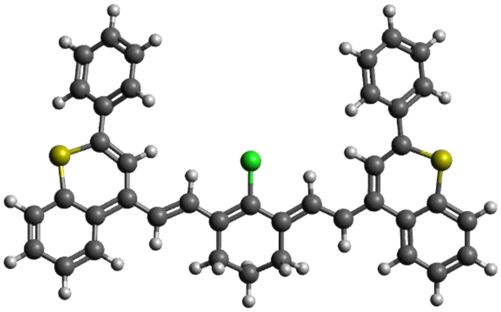

| | | | |
|---|---|---|---|
| 73 | | | |
| C | -0.2094099300 | -1.4309148688 | -0.3059655963 |
| C | -1.3627576757 | -2.2281289464 | -0.2463725433 |
| C | 1.0278186926 | -1.8634904205 | -0.8070844039 |
| C | -1.2775609128 | -3.6249988096 | -0.7981020471 |
| C | -0.2390641213 | -3.7350171303 | -1.8950844607 |
| H | -2.2525304471 | -3.9215668958 | -1.1871428766 |
| H | -1.0379804220 | -4.3229466094 | 0.0135413775 |
| C | 1.1062294479 | -3.2422309023 | -1.4052278018 |
| H | 1.5105110816 | -3.9376470853 | -0.6597513515 |
| H | 1.8148680156 | -3.2322641065 | -2.2352815813 |
| H | -0.5560862704 | -3.1345748494 | -2.7526296338 |
| H | -0.1597398013 | -4.7676275621 | -2.2387127470 |
| Cl | -0.3102624897 | 0.1876516337 | 0.3157414692 |
| C | 2.1639548970 | -1.0627673753 | -0.7279530912 |
| C | 3.4342288539 | -1.4340610805 | -1.1393448177 |
| C | -2.5424760934 | -1.7575706484 | 0.3226326916 |
| C | -3.6996642689 | -2.4978239028 | 0.5046535967 |
| H | 2.0225911186 | -0.0855003990 | -0.2889598928 |
| C | 4.5915953601 | -0.6492571147 | -1.0318515720 |
| C | 4.5237624167 | 0.6448461059 | -0.4625701183 |
| C | 5.8714340471 | -1.1550271898 | -1.5095920368 |
| C | 5.5602195310 | 1.4846782158 | -0.1923662934 |
| C | 7.0701821167 | -0.4397599562 | -1.3237846805 |
| S | 7.1878794815 | 1.0864487097 | -0.5207181300 |
| H | 3.5461491187 | 1.0327855937 | -0.2136410413 |
| C | 5.9734860960 | -2.3792469004 | -2.1947482535 |
| C | 8.2940441422 | -0.9439695738 | -1.7736230831 |
| C | 7.1760536818 | -2.8710570171 | -2.6408059566 |
| C | 8.3508021308 | -2.1529601538 | -2.4233891727 |
| H | 5.0836707110 | -2.9565124927 | -2.3956971923 |
| H | 7.2073139198 | -3.8169990811 | -3.1657955816 |
| H | 6.5602859943 | 5.9634371423 | 0.4033263021 |
| C | 5.9515850202 | 5.1170149913 | 0.6948751163 |
| C | 4.9734124385 | 5.2644276933 | 1.6669502722 |
| H | 4.8233609407 | 6.2247472936 | 2.1439707140 |
| C | 4.1911529136 | 4.1772556734 | 2.0307936411 |
| H | 3.4374647755 | 4.2838826247 | 2.8007807878 |

| | | | |
|---|---|---|---|
| C | 4.3825451198 | 2.9494579710 | 1.4244984793 |
| H | 3.7944475158 | 2.0958724206 | 1.7381057142 |
| C | 5.3623272963 | 2.7925188932 | 0.4420012018 |
| C | 6.1492576496 | 3.8894703425 | 0.0877322861 |
| H | 6.9002793960 | 3.7875708723 | -0.6864311682 |
| C | -4.9029480009 | -2.0107136331 | 1.0365385087 |
| C | -5.0513924541 | -0.6293256219 | 1.3048472434 |
| C | -6.0200704969 | -2.9131723860 | 1.2783813530 |
| C | -7.2756659659 | -2.4444782285 | 1.7105942399 |
| C | -6.1666486720 | 0.0119813328 | 1.7510005937 |
| S | -7.6347115001 | -0.7944592735 | 2.0797981140 |
| H | -4.2147310579 | 0.0175972481 | 1.0815933052 |
| C | -8.3480918347 | -3.3189460964 | 1.9103453314 |
| C | -5.8999492145 | -4.3026331030 | 1.0956439227 |
| C | -8.1922116363 | -4.6678646721 | 1.7027377956 |
| C | -6.9521125668 | -5.1615877302 | 1.3006037176 |
| H | -6.8132344619 | -6.2247472936 | 1.1530326958 |
| H | -4.9508039565 | -4.7231956204 | 0.7995819903 |
| H | -6.2181623235 | 5.2784063437 | 2.6028411059 |
| C | -6.2108328017 | 4.2097559752 | 2.4290934870 |
| C | -7.3304580324 | 3.5840916021 | 1.9015723172 |
| H | -8.2108537390 | 4.1632021762 | 1.6535775985 |
| C | -7.3250499774 | 2.2178113443 | 1.6827023316 |
| C | -6.1921258874 | 1.4603315791 | 1.9825386155 |
| C | -5.0712674805 | 2.0976428080 | 2.5178196287 |
| H | -4.2015467025 | 1.5135095502 | 2.7922896213 |
| C | -5.0829728956 | 3.4625633883 | 2.7386942574 |
| H | -4.2125964156 | 3.9445811203 | 3.1657955816 |
| H | -2.5230128282 | -0.7341077719 | 0.6690763569 |
| H | -3.6677532478 | -3.5363431595 | 0.2145859254 |
| H | 3.5429112646 | -2.4258664387 | -1.5492220394 |
| H | 9.1969751213 | -0.3684789489 | -1.6069186836 |
| H | -8.1951610755 | 1.7397190439 | 1.2487613280 |
| H | -9.3015581128 | -2.9213746963 | 2.2376087256 |
| H | 9.3015581128 | -2.5367518164 | -2.7701642734 |
| H | -9.0259070220 | -5.3397672371 | 1.8609243886 |

## References


(1) Gasevic, T.; Stückrath, J. B.; Grimme, S.; Bursch, M. Optimization of the R2SCAN-3c Composite Electronic-Structure Method for Use with Slater-Type Orbital Basis Sets. *J. Phys. Chem. A* **2022**, *126* (23), 3826–3838. https://doi.org/10.1021/acs.jpca.2c02951.

(2) Grimme, S.; Hansen, A.; Ehlert, S.; Mewes, J. M. R2SCAN-3c: A “Swiss Army Knife” Composite Electronic-Structure Method. *J. Chem. Phys.* **2021**, *154* (6). https://doi.org/10.1063/5.0040021.

(3) Weigend, F. Accurate Coulomb-Fitting Basis Sets for H to Rn. *Phys. Chem. Chem. Phys.* **2006**, *8* (9), 1057–1065. https://doi.org/10.1039/b515623h.

(4) Weigend, F.; Ahlrichs, R. Balanced Basis Sets of Split Valence, Triple Zeta Valence and Quadruple Zeta Valence Quality for H to Rn: Design and Assessment of Accuracy. *Phys. Chem. Chem. Phys.* **2005**, *7* (18), 3297–3305. https://doi.org/10.1039/b508541a.

(5) Neese, F.; Wennmohs, F.; Becker, U.; Riplinger, C. The ORCA Quantum Chemistry Program Package. *J. Chem. Phys.* **2020**, *152* (22). https://doi.org/10.1063/5.0004608.

(6) Neese, F. Software Update: The ORCA Program System—Version 5.0. *Wiley Interdiscip. Rev. Comput. Mol. Sci*. John Wiley and Sons Inc September 1, 2022. https://doi.org/10.1002/wcms.1606.

(7) Cosco, E. D.; Caram, J. R.; Bruns, O. T.; Franke, D.; Day, R. A.; Farr, E. P.; Bawendi, M. G.; Sletten, E. M. Flavylium Polymethine Fluorophores for Near- and Shortwave Infrared Imaging. *Angew. Chem.* **2017**, *129* (42), 13306–13309. https://doi.org/10.1002/ange.201706974.

(8) Heng, H.; Song, G.; Cai, X.; Sun, J.; Du, K.; Zhang, X.; Wang, X.; Feng, F.; Wang, S. Intrinsic Mitochondrial Reactive Oxygen Species (ROS) Activate the In Situ Synthesis of Trimethine Cyanines in Cancer Cells. *Angew. Chem. Int. Ed.* **2022**, *61* (38). https://doi.org/10.1002/anie.202203444.

(9) Langhals, H.; Varja, A.; Laubichler, P.; Kernt, M.; Eibl, K.; Haritoglou, C. Cyanine Dyes as Optical Contrast Agents for Ophthalmological Surgery. *J. Med. Chem.* **2011**, *54* (11), 3903–3925. https://doi.org/10.1021/jm2001986.

(10) Gamage, R. S.; Smith, B. D. Fluorescence Imaging Using Deep-Red Indocyanine Blue, a Complementary Partner for Near-Infrared Indocyanine Green. *CBMI* **2024**. https://doi.org/10.1021/cbmi.4c00008.

(11) Swamy, M. M. M.; Murai, Y.; Monde, K.; Tsuboi, S.; Swamy, A. K.; Jin, T. Biocompatible and Water-Soluble Shortwave-Infrared (SWIR)-Emitting Cyanine-Based Fluorescent Probes for In Vivo Multiplexed Molecular Imaging. *ACS Appl. Mater. Interfaces* **2024**, *16* (14), 17253–17266. https://doi.org/10.1021/acsami.4c01000.

(12) Friedman, H. C.; Cosco, E. D.; Atallah, T. L.; Jia, S.; Sletten, E. M.; Caram, J. R. Establishing Design Principles for Emissive Organic SWIR Chromophores from Energy Gap Laws. *Chem* **2021**, *7* (12), 3359–3376. https://doi.org/10.1016/j.chempr.2021.09.001.
